# Supplementary material for: Artificial neural network solver for Fokker-Planck and Koopman eigenfunctions
Source: arXiv:2508.20339 source file (2025-08-28)
Supplement: Supplementary file 1 [file supplementary_material.pdf]

# SUPPLEMENTARY MATERIALS: Artificial neural network solver for Fokker-Planck and Koopman eigenfunctions

Max Kreider*†, Peter J. Thomas‡, and Yao Li§

## SM1. Algorithms.

Here, we include algorithms and further implementation details for our machine learning approach to compute SKO and Fokker-Planck eigenfunctions. Our approach relies on Monte Carlo simulation of an Itô SDE (see (2.1) in the main text):

$$d\mathbf{X} = \mathbf{f}(\mathbf{X})dt + \mathbf{g}(\mathbf{X})d\mathbf{W}(t) \quad \text{(SM1.1)}$$

Unless otherwise stated, we utilize the Euler-Maruyama method to generate realizations of the process (SM1.1) [SM8]. We implement all algorithms stated in this section in C++.

### SM1.1. Step 1: Collocation points.

For clarity, here we recapitulate the text in the main document. The exposition is then augmented with Algorithms (SM1.1) and (SM1.2) which provide pseudocode and further implementation details.

Here, the goal is to generate two sets of collocation points: $\mathcal{X} = \{\mathbf{x}_i,\ i = 1, 2, \ldots, N_x\}$ and $\mathcal{Y} = \{\mathbf{y}_j,\ j = 1, 2, \ldots, N_y\}$. We call $\mathcal{X}$ the "training set" and $\mathcal{Y}$ the "reference set". Ultimately, a neural network will learn a specific eigenfunction on the training set to replace boundary conditions, and will learn the differential operator, $\mathcal{L}$ or $\mathcal{L}^\dagger$, on the reference set. In other words, training on $\mathcal{Y}$ ensures that the output of the ANN satisfies (approximately) either the forward or backward equation, while training on $\mathcal{X}$ guides the ANN to a specific normalization of an eigenfunction and avoids the trivial solution.

To generate the training set, $\mathcal{X}$, we discretize the rectangular computational domain $\mathcal{R}$ into boxes of equal dimension, but we store in memory only $N_x$ of the boxes corresponding to the chosen collocation points. Each box is represented by the coordinates corresponding to the center of the respective box. This step is critical in higher dimensions, where storing a full mesh is not feasible. The points, $\mathbf{x}_i$, at the centers of the boxes will be associated with numerical estimates of the probability density. In contrast, we do not bin the reference set in boxes because these points are used solely for minimizing the residual of the operator loss.

The support of the forward eigenmodes is often restricted to the invariant distribution, which may be concentrated near low dimensional manifolds or in specific regions of the domain. While to the best of our knowledge this is not supported by known results, we expect concentration results of invariant probability measures [SM5, SM6, SM12] and quasi-stationary distributions [SM17] to be applicable after some modifications. In contrast, the support of the backward eigenmodes typically spans all of $\Omega$. The generation of the collocation points should take this difference into account.

To generate collocation points, $\mathcal{X}$, we first run (SM1.1) for a "burn-in" time, $T_{\text{burn}}$, so that the location of the terminal point of the process is effectively drawn from a distribution

*Department of Mathematics, Applied Mathematics, and Statistics, Case Western Reserve University.
†Corresponding author: mbk62@case.edu
‡Department of Mathematics, Applied Mathematics, and Statistics, Case Western Reserve University.
§Department of Mathematics and Statistics, University of Massachusetts Amherst



This manuscript is for review purposes only.

that is near the stationary distribution. Then, we choose a "ratio", $\alpha \in [0, 1]$, continue the realization of (SM1.1) starting from the terminal point of the burn-in simulation, and take only a fraction $\alpha$ (one should generally take $\alpha \in [0.5, 0.9]$) of the collocation points from this trajectory. We establish a "sample" time, $t_{\text{gap}}$, and sample only at integer multiples of $t_{\text{gap}}$ so that points are not too close to each other. The other $1 - \alpha$ of the collocation points are chosen from a uniform distribution on the computational domain $\mathcal{R}$. We associate each sampled point $\mathbf{x}_i$ with the box in $\mathcal{R}$ in which it lands provided it has not yet been taken by a collocation point. The process stops when $N_x$ collocation points are collected. We reiterate that only points $\mathbf{x}_i$ are binned in the boxes, and that one should take $\alpha = 0$ when generating collocation points for the backward eigenmodes. This procedure ensures that many of the collocation points are in locations where the forward eigenmodes take on non-trivial values, and ultimately reduces the number of collocation points required for accurate estimation.

A similar procedure can be used to generate $\mathcal{Y}$, although these points are not binned in boxes because they are used to evaluate the differential operator and are not associated with numerical estimates of a probability density. Algorithms (SM1.1) and (SM1.2) provide more details for the generation of $\mathcal{Y}$ and $\mathcal{X}$, respectively [SM20].

**Algorithm SM1.1** Collocation point generation for $\mathcal{Y}$

**Input:** ratio $\alpha \in [0, 1]$, domain $\mathcal{R}$, initial condition $\mathbf{X}_0$, burn-in time $T_{\text{burn}}$, sampling gap $t_{\text{gap}}$
**Output:** $\mathcal{Y} = \{\mathbf{y}_j,\ j = 1, 2, \ldots, N_y\}$

Run a numerical trajectory of (SM1.1) with initial condition $\mathbf{X}_0$ until time $T_{\text{burn}}$;

**for** $j = 1$ to $N_y$ **do**
  Generate a random number $\xi \sim U([0, 1])$;
  **if** $\xi < \alpha$ **then**
    Let $t_j = t_{j-1} + t_{\text{gap}}$;
    Run a numerical trajectory of (SM1.1) until time $t_j$;
    Let $\mathbf{y}_j = \mathbf{X}(t_j)$;
  **else**
    Let $t_j = t_{j-1}$;
    Generate a random point $\mathbf{y}_j \sim U(\mathcal{R})$;
  **end if**
**end for**

**return** $\mathcal{Y} = \{\mathbf{y}_j,\ j = 1, 2, \ldots, N_y\}$;

*This manuscript is for review purposes only.*

**Algorithm SM1.2** Collocation point generation for $\mathcal{X}$

**Input:** ratio $\alpha \in [0, 1]$, domain $\mathcal{R}$, initial condition $\mathbf{X}_0$, burn-in time $T_{\text{burn}}$, sampling gap $t_{\text{gap}}$
**Output:** $\mathcal{X} = \{\mathbf{x}_i,\ i = 1, 2, \ldots, N_x\}$

Run a numerical trajectory of (SM1.1) with initial condition $\mathbf{X}_0$ until time $T_{\text{burn}}$;
Set count $i = 1$;

**while** $i < N_x$ **do**

  Generate a random number $\xi \sim U([0, 1])$;

  **if** $\xi < \alpha$ **then**
    Let $t_i = t_{i-1} + t_{\text{gap}}$;
    Continue the numerical trajectory of (SM1.1) until time $t_i$;
    Map state to corresponding box: $\mathbf{X}(t_i) \to \mathbf{x}$;
  **else**
    Let $t_i = t_{i-1}$;
    Generate a random point $\mathbf{x}' \sim U(\mathcal{R})$;
    Map state to corresponding box: $\mathbf{x}' \to \mathbf{x}$;
  **end if**

  **if** $\mathbf{x}$ is not flagged **then**
    Set $\mathbf{x}_i = \mathbf{x}$;
    Flag $\mathbf{x}_i$;
    Set $i = i + 1$;
  **end if**

**end while**

**return** $\mathcal{X} = \{\mathbf{x}_i,\ i = 1, 2, \ldots, N_x\}$;

**SM1.2. Step 2: density estimation.** For clarity, here we recapitulate the text in the main document. The exposition is then augmented with Algorithms (SM1.3) and (SM1.4) which provide pseudocode and further implementation details.

The goal of this step is to estimate time-dependent probability densities associated with (SM1.1). To numerically approximate a time-dependent density, we fix a sampling time interval, $t_{\text{gap}}$, and the number of sample times, $N_t$. Realizations of the process (SM1.1) are sampled at integer multiples of $t_{\text{gap}}$ so that samples are not too close together.[1] These samples are recorded in a matrix $\mathcal{D}$, which has $N_t$ rows (one for each time slice) and $N_x$ columns (one for each collocation point, $\mathbf{x}_i \in \mathcal{X}$).

The procedures for estimating the densities associated with forward and backward eigenfunctions differ. To distinguish between them, we denote by $\mathcal{D}_F$ and $\mathcal{D}_B$ the matrices containing the estimated time-dependent densities for the forward and backward eigenfunctions, respectively.

We begin by estimating the forward transition densities $\rho(\mathbf{x}_i, t_k \mid \mathbf{x}_0, 0)$ for a fixed initial condition $\mathbf{x}_0$, where $\mathbf{x}_i \in \mathcal{X}$ and $t_k \in t_1, \ldots, t_{N_t}$. Using Monte Carlo simulation, we generate $K$ realizations of equation (SM1.1) starting from $\mathbf{x}_0$. At each sampling time $t_k$, we count how many trajectories fall into the bin centered at each collocation point $\mathbf{x}_i$. If the bin around $\mathbf{x}_i$ contains $K_i$ samples, the estimated transition probability is given by $K_i/(K\delta_i)$, where $\delta_i$ is the volume of the bin around $\mathbf{x}_i$. These estimated values are then stored in the matrix $\mathcal{D}_F$.

Letting $\tilde{\rho}_{f,i}(t_k) \equiv \tilde{\rho}(\mathbf{x}_i, t_k \mid \mathbf{x}_0, 0)$ denote the estimated transition density, it follows that the $i$th column of $\mathcal{D}_F$ provides an approximation to the time series $\tilde{\rho}_{f,i}(t_k)_{k=1}^{N_t}$. Since the initial condition $\mathbf{x}_0$ is fixed, the coefficient $Q^*_{\lambda_1}(\mathbf{x}_0)$ in the eigenfunction expansion ansatz is constant. If desired, one can also sample $\mathbf{x}_0$ from a prescribed distribution to reduce the influence of higher-order modes. Algorithm SM1.3 contains more details.

We now turn to the computation of the backward eigenmodes. The objective in this step is to approximate the forward transition probability $\rho(\mathcal{B}, t \mid \mathbf{x}_i, 0)$ for each $\mathbf{x}_i \in \mathcal{X}$ at a sequence of time points $\mathbf{t} = \{t_k\}_{k=1}^{N_t}$. Here, $\mathcal{B}$ denotes a reference box, $\mathcal{B} \subset \mathcal{R}$, which is chosen to contain a nontrivial portion of the invariant density.[2] We denote the estimated transition probability into $\mathcal{B}$ at time $t_k$, given initial condition $\mathbf{x}_i$, by $\tilde{\rho}_{b,i}(t_k) \equiv \tilde{\rho}(\mathcal{B}, t_k \mid \mathbf{x}_i, 0)$.

To compute $\tilde{\rho}(\mathcal{B}, t_k \mid \mathbf{x}_i, 0)$, we simulate $K$ realizations of equation (SM1.1), all initialized at $\mathbf{x}_i$. For each time $t_k$, we count the number of trajectories, say $K_j$, that lie within the set $\mathcal{B}$. The estimated transition probability is then given by $\tilde{\rho}_{b,i}(t_k) = K_j/K$, and the result is stored in the matrix $\mathcal{D}_B$. In our numerical examples, approximately $N_{\text{sample}} = 10^4$ trajectories per $\mathbf{x}_i$ are sufficient to achieve accurate estimates. Additional implementation details are provided in Algorithm SM1.4. It is important to note that in estimating $\tilde{\rho}_{b,i}(t_k)$, the terminal region $\mathcal{B}$ is fixed. As a result, in the eigenfunction expansion ansatz, the integrals $\int_{\mathcal{B}} d\mathbf{y}\; P_{\lambda_1}(\mathbf{y})$ and $\int_{\mathcal{B}} d\mathbf{y}\; P_0(\mathbf{y})$ remain constant across all initial conditions $\mathbf{x}_i$. This property is exploited in Step 4 (see the main text) to recover the backward eigenfunctions over the domain $\mathcal{X}$.

[1]The parameter $t_{\text{gap}}$ should be much smaller than the mean period of oscillation of a given system.

[2]The reference box is introduced as a practical approximation. Ideally, one would track the probability mass arriving in an individual box, but the likelihood of a trajectory landing in a single small bin is typically very low, necessitating a prohibitively large number of samples. To improve sampling efficiency, we instead consider a larger region $\mathcal{B}$.

**Algorithm SM1.3** Density estimation for forward eigenmodes

```
Input: Collocation points 𝒳, initial box x_0 ∈ ℛ, sampling gap t_gap, timestep dt, number of sample times N_t, number of samples K, uniform bin size δ
Output: Forward data matrix 𝒟_F

for i = 1 to K do
    Generate starting point x_IC ~ U(x_0);
    for j = 0 to N_t · t_gap do
        Run (SM1.1) for one timestep with initial condition x_IC to output X_dt;
        Set x_IC = X_dt;
        if mod(j, t_gap) = 0 and X_dt lands in one of the N_x boxes then
            Set I as the index of the box;
            Increment 𝒟(j, I) by 1/(Kδ);
        end if
    end for
end for

return Forward data matrix 𝒟_F;
```

**Algorithm SM1.4** Density estimation for backward eigenmodes

```
Input: collocation points 𝒳, sampling interval t_gap, timestep dt, number of sample times N_t, number of samples K, reference box ℬ
Output: Backward data matrix 𝒟_B

for i = 0 to N_x do
    for k = 0 to K do
        Set x_IC = x_i;
        for j = 0 to N_t · t_gap do
            Run (SM1.1) for one timestep with initial condition x_IC to output X_dt;
            if mod(j, t_gap) = 0 and X_dt lies inside ℬ then
                Set I as the index of the x_i;
                Increment 𝒟(j, I) by 1/K;
            end if
            Set x_IC = X_dt;
        end for
    end for
end for

return Backward data matrix 𝒟_B;
```

## SM2. Artificial Neural Network (ANN) Details.

In this section, we provide further details pertaining to the implementation of an artificial neural network (ANN) for step 5 in the main text. We use multilayer feedforward neural networks, which are compositions of functions [SM1]:

$$\mathcal{N}(\mathbf{x};\chi) = W^L\sigma^L(W^{L-1}\sigma^{L-1}(\dots\sigma^1(W^0\mathbf{x}+b^0)\dots)+b^{L-1})+b^L \tag{SM2.1}$$

where $W^\ell$ are weight matrices and $b^\ell$ are bias vectors for $\ell = 0,1,2,\dots,L$, and $\mathbf{x}$ is the vector of state variables, i.e., network inputs.

Unless otherwise specified, we fix $L = 5$ so that our ANN has six layers (input, output, and $L-1 = 4$ hidden layers). For $\ell = 0,1,\dots,5$, we take $W^\ell \in \mathbb{R}^{90\times d_\ell}$ and $b^\ell \in \mathbb{R}^{90}$, where $d_0 = n$ is the input dimension, and $d_\ell = 90$ for $\ell \geq 1$. We take $n = 2,3,4$ depending on the dimension of the problem. The final output layer has $W^6 \in \mathbb{R}^{m\times 90}$ and $b^6 \in \mathbb{R}^m$, where $m$ is the output dimension. We take $m = 2$ to represent the real and imaginary parts of an eigenfunction. The hidden layers are fully connected with sigmoid activation functions, while the output layer has no associated nonlinearity. We form and train the network using TensorFlow 2 [SM4].

## SM3. Error Decomposition of Eigenfunction Approximation.

In this section, we restate and prove Lemma 1 pertaining to the error decomposition of our least-squares approach to approximating the eigenfunctions of the forward operator and SKO.

Lemma SM3.1. *Assume the real parts of $M$ known eigenvalues satisfy $0 > \mu_1 > \cdots \mu_M$ and $\hat{\lambda}^\pm = \hat{\mu} \pm i\,\hat{\omega}$ is a known high-order eigenvalue satisfying $|\hat{\mu}| > |\mu_i|$ and $|\hat{\omega}| > |\omega_i|$ for each $i = 1,\cdots,M$. Let the time slices $\{t_j\}_{j=1}^N$ be an equipartition of $[T_s, T_f]$ for $N$ sufficiently large. If Monte Carlo error terms $\{\varepsilon_i\}_{i=1}^N$ are i.i.d. standard normal random variables, then we have*

$$\|\beta - \beta_0\| \leq \mathcal{O}(|\mu_1+\hat{\mu}|^{-1}e^{(\hat{\mu}-\mu_1)T_s}) + \mathcal{O}(N^{-1/2}e^{-\mu_1 T_s}) \tag{SM3.1}$$

*Proof.* The solution to the least square problem is

$$\beta = (\mathscr{X}^T\mathscr{X})^{-1}\mathscr{X}^T\mathscr{Y} \tag{SM3.2}$$

therefore we may decompose the solution as

$$\beta - \beta_0 = \beta_\varepsilon + \beta_h \tag{SM3.3}$$

for

$$\beta_\varepsilon = (\mathscr{X}^T\mathscr{X})^{-1}\mathscr{X}^T D\varepsilon \tag{SM3.4}$$

and

$$\beta_h = (\mathscr{X}^T\mathscr{X})^{-1}\mathscr{X}^T\mathscr{Y}_h \tag{SM3.5}$$

Notice that terms in $\mathscr{X}^T\mathscr{X}$ satisfy

(SM3.6)

$$
\begin{aligned}
(\mathscr{X}^T\mathscr{X})_{2i-1,2j-1} &= \sum_{i=1}^{N} e^{(\mu_i+\mu_j)t_k}\cos(\omega_i t_k)\cos(\omega_j t_k)\\
=&N\left(\int_{T_s}^{T_f} e^{(\mu_i+\mu_j)t}\cos(\omega_i t)\cos(\omega_j t)\;dt+\mathcal{O}(1/N)\right)\\
=&\frac{N}{2}\left[\frac{e^{(\mu_i+\mu_j)t}}{(\mu_i+\mu_j)^2+(\omega_i-\hat{\omega})^2}\left((\mu_i+\mu_j)\cos((\omega_i-\hat{\omega})t)+(\omega_i-\hat{\omega})\sin((\omega_i-\hat{\omega})t)\right)\Bigg|_{T_s}^{T_f}\right.\\
&\left.+\frac{e^{(\mu_i+\mu_j)t}}{(\mu_i+\mu_j)^2+(\omega_i+\hat{\omega})^2}\left((\mu_i+\mu_j)\cos((\omega_i+\hat{\omega})t)+(\omega_i+\hat{\omega})\sin((\omega_i+\hat{\omega})t)\right)\Bigg|_{T_s}^{T_f}+\mathcal{O}(1/N)\right]\\
=&Ne^{2\mu_1 T_s}(\mathbf{H}_{2i-1,2j-1}(\mu_i,\mu_j,T_s,T_f)+\mathcal{O}(1/N))
\end{aligned}
$$

for an $\mathcal{O}(1)$ function $\mathbf{H}_{2i-1,2j-1}$ that only depends on $\lambda_i,\lambda_j,T_s$, and $T_f$. Similar calculation gives

$$
\begin{aligned}
(\mathscr{X}^T\mathscr{X})_{2i-1,2j} &= Ne^{2\mu_1 T_s}(\mathbf{H}_{2i-1,2j}(\mu_i,\mu_j,T_s,T_f)+\mathcal{O}(1/N))\\
(\mathscr{X}^T\mathscr{X})_{2i,2j-1} &= Ne^{2\mu_1 T_s}(\mathbf{H}_{2i,2j-1}(\mu_i,\mu_j,T_s,T_f)+\mathcal{O}(1/N))
\end{aligned}
\tag{SM3.7}
$$

and

$$
(\mathscr{X}^T\mathscr{X})_{2i,2j} = Ne^{2\mu_1 T_s}(\mathbf{H}_{2i,2j}(\mu_i,\mu_j,T_s,T_f)+\mathcal{O}(1/N))
\tag{SM3.8}
$$

Therefore, we have $\mathscr{X}^T\mathscr{X} = N(e^{2\mu_1 T_s}\mathbf{H}+\mathcal{O}(1/N))$ for a matrix $\mathbf{H}$ that only depends on the leading $M$ eigenvalues and $T_s$, $T_f$.

We also have

$$
\begin{aligned}
(\mathscr{X}^T\mathscr{Y})_{2i-1} &= \sum_{i=1}^{N} e^{(\mu_i+\hat{\mu})t_k}\cos(\omega_i t_k)\cos(\hat{\omega}t_k+\phi)\\
&= N\left(\int_{T_s}^{T_f} e^{(\mu_i+\hat{\mu})t}\cos(\omega_i t)\cos(\hat{\omega}t+\phi)\;dt+\mathcal{O}(1/N)\right)
\end{aligned}
\tag{SM3.9}
$$

and

$$
\begin{aligned}
(\mathscr{X}^T\mathscr{Y})_{2i} &= \sum_{i=1}^{N} e^{(\mu_i+\hat{\mu})t_k}\sin(\omega_i t_k)\cos(\hat{\omega}t_k+\phi)\\
&= N\left(\int_{T_s}^{T_f} e^{(\mu_i+\hat{\mu})t}\sin(\omega_i t)\cos(\hat{\omega}t+\phi)\;dt+\mathcal{O}(1/N)\right)
\end{aligned}
\tag{SM3.10}
$$

*This manuscript is for review purposes only.*

Similar calculation of entries of $\mathscr{X}^T\mathscr{Y}$ gives

(SM3.11)

$$
\begin{aligned}
&\int_{T_s}^{T_f} e^{(\mu_i+\hat{\mu})t}\sin(\omega_i t)\cos(\hat{\omega}t+\phi)\,dt\\
=&\frac{1}{2}\left[\frac{e^{(\mu_i+\hat{\mu})t}}{(\mu_i+\hat{\mu})^2+(\omega_i-\hat{\omega})^2}\left((\mu_i+\hat{\mu})\cos((\omega_i-\hat{\omega})t-\phi)+(\omega_i-\hat{\omega})\sin((\omega_i-\hat{\omega})t-\phi)\right)\Big|_{T_s}^{T_f}\right.\\
&\left.+\frac{e^{(\mu_i+\hat{\mu})t}}{(\mu_i+\hat{\mu})^2+(\omega_i+\hat{\omega})^2}\left((\mu_i+\hat{\mu})\cos((\omega_i+\hat{\omega})t+\phi)+(\omega_i+\hat{\omega})\sin((\omega_i+\hat{\omega})t+\phi)\right)\Big|_{T_s}^{T_f}\right]\\
\le&\frac{1}{2}\left[e^{(\mu_i+\hat{\mu})T_s}-e^{(\mu_i+\hat{\mu})T_f}\right]\left[\frac{|\mu_i+\hat{\mu}|+|\omega_i-\hat{\omega}|}{(\mu_i+\hat{\mu})^2+(\omega_i-\hat{\omega})^2}+\frac{|\mu_i+\hat{\mu}|+|\omega_i+\hat{\omega}|}{(\mu_i+\hat{\mu})^2+(\omega_i+\hat{\omega})^2}\right]\\
\le&e^{(\mu_1+\hat{\mu})T_s}e^{(\mu_i-\mu_1)T_s}\left(\frac{1}{|\mu_i+\hat{\mu}|+|\omega_i-\hat{\omega}|}+\frac{1}{|\mu_i+\hat{\mu}|+|\omega_i+\hat{\omega}|}\right)\\
\le&\frac{2e^{(\mu_1+\hat{\mu})T_s}}{|\mu_1+\hat{\mu}|}
\end{aligned}
$$

and also

(SM3.12) $$\int_{T_s}^{T_f} e^{(\mu_i+\hat{\mu})t}\cos(\omega_i t)\cos(\hat{\omega}t+\phi)\,dt \le \frac{2e^{(\mu_1+\hat{\mu})T_s}}{|\mu_1+\hat{\mu}|}$$

Therefore, when $\hat{\mu}$ is sufficiently large, by solving the normal equation $\beta_h = (\mathscr{X}^T\mathscr{X})^{-1}\mathscr{X}^T\mathscr{Y}_h$, we have $\|\beta_h\| \le \mathcal{O}(|\mu_1+\hat{\mu}|^{-1}e^{(\hat{\mu}-\mu_1)T_s}) + \mathcal{O}(1/N)$.

It remains to estimate $\|\beta_\varepsilon\|$. Since entries of $\varepsilon$ are i.i.d. normal random variables, we have

$$\mathbb{E}[\|\varepsilon\|^2] = \epsilon^2\mathrm{Tr}(Z^TZ)$$

for $Z = (\mathscr{X}^T\mathscr{X})^{-1}\mathscr{X}D$. Notice that $Z^TZ$ and $ZZ^T$ have the same trace. Some calculation gives $\mathrm{Tr}(Z^TZ) = \mathrm{Tr}(D^2(\mathscr{X}^T\mathscr{X})^{-1}))$. Recall that $D$ is an $\mathcal{O}(1)$ matrix determined by $\{p_f(t_i)\}$. Since $\mathscr{X}^T\mathscr{X} = N(e^{2\mu_1T_s}\mathbf{A}+\mathcal{O}(1/N))$ for an $\mathcal{O}(1)$ matrix $\mathbf{A}$, we have $\|\beta_\varepsilon\| = \mathcal{O}(e^{-\mu_1T_s}N^{-1/2})$. Notice that $\mathcal{O}(1/N)$ is absorbed by $\mathcal{O}(N^{-1/2})$. This completes the proof. ■

**SM4. Finite Differences.** In this section, our goal is to discretize the backward operator using finite difference (FD) methods as a means to gauge the accuracy of our machine learning approach.[3] We will apply the FD framework to approximate the eigenvalues and eigenfunctions of two-dimensional stochastic oscillators, assumed to admit adjoint-reflecting boundary conditions. In two dimensions, adjoint-reflecting boundary conditions simplify to vanishing Neumann conditions [SM3].

[3] Finite difference methods have been used in previous works to accurately compute the eigenfunctions of 2D stochastic oscillators [SM15, SM16].

We begin by stating the problem, along with a brief derivation of the FD methods that we employ. We consider elliptic PDEs of the form

$$m(x,y)\partial_x u(x,y) + n(x,y)\partial_y u(x,y) + f(x,y)\partial_{xx} u(x,y) + g(x,y)\partial_{yy} u(x,y) = 0 \tag{SM4.1}$$

on a rectangular domain

$$\Omega = \{(x,y) \mid a \le x \le b,\ c \le y \le d\} \tag{SM4.2}$$

In all cases, we assume vanishing Neumann conditions on the boundary

$$\frac{\partial u}{\partial \mathbf{n}} = 0 \text{ on } \partial\Omega \tag{SM4.3}$$

where $\mathbf{n}$ is the outward normal vector on $\partial\Omega$. We discretize the $x$ and $y$-directions uniformly according to

$$h = \frac{b-a}{\mathcal{I}}, \quad k = \frac{d-c}{\mathcal{J}} \tag{SM4.4}$$

for fixed integers $\mathcal{I}, \mathcal{J} \in \mathbb{N}$. Then, we define a grid

$$\begin{aligned} x_i &= a + ih, \quad i = 0,1,2,\dots,\mathcal{I} \\ y_j &= c + jk, \quad j = 0,1,2,\dots,\mathcal{J} \end{aligned} \tag{SM4.5}$$

We introduce the notation $f_{i,j} \equiv f(x_i, y_j)$ and so forth for the other functions in (SM4.1). To discretize (SM4.1), we employ standard 2nd order centered difference schemes

$$\begin{aligned} \partial_x u(x_i,y_j) &= \frac{-u_{i-1,j} + u_{i+1,j}}{2h} + \mathcal{O}(h^2) \\ \partial_y u(x_i,y_j) &= \frac{-u_{i,j-1} + u_{i,j+1}}{2k} + \mathcal{O}(k^2) \\ \partial_{xx} u(x_i,y_j) &= \frac{u_{i-1,j} - 2u_{i,j} + u_{i+1,j}}{h^2} + \mathcal{O}(h^2) \\ \partial_{yy} u(x_i,y_j) &= \frac{u_{i,j-1} - 2u_{i,j} + u_{i,j+1}}{k^2} + \mathcal{O}(k^2) \end{aligned} \tag{SM4.6}$$

Leveraging (SM4.6), we rewrite (SM4.1) as a difference equation of the form

(SM4.7)
$$\begin{aligned} -\frac{1}{h^2}\Bigg( \left[\frac{h}{2}m_{i,j} - f_{i,j}\right] w_{i-1,j} + \left[\frac{h^2}{2k}n_{i,j} - \frac{h^2}{k^2}g_{i,j}\right] w_{i,j-1} + \left[2f_{i,j} + \frac{h^2}{k^2}g_{i,j}\right] w_{i,j} \\ + \left[-\frac{h^2}{2k}m_{i,j} - \frac{h^2}{k^2}g_{i,j}\right] w_{i,j+1} + \left[-\frac{h}{2}m_{i,j} - f_{i,j}\right] w_{i+1,j} \Bigg) = 0 \end{aligned}$$

where each $w_{i,j}$ is an approximation of $u_{i,j}$. We remark that (SM4.7) is valid for the interior points $i = 1,2,\dots,\mathcal{I}-1$ and $j = 1,2,\dots,\mathcal{J}-1$.

It remains to account for the vanishing Neumann conditions on the boundary: $i = 0, \mathcal{I}$ and $j = 0, \mathcal{J}$. We first rewrite (SM4.7) in block tridiagonal form, and then discuss proper implementation of boundary conditions.

To that end, we introduce the notation

$$\mathbf{z} = \begin{bmatrix} \mathbf{z}_0 \\ \vdots \\ \mathbf{z}_i \\ \vdots \\ \mathbf{z}_{\mathcal{I}} \end{bmatrix}, \quad \mathbf{z}_i = \begin{bmatrix} w_{i,0} \\ w_{i,1} \\ \vdots \\ w_{i,\mathcal{J}} \end{bmatrix} \tag{SM4.8}$$

and define the block matrix

$$\mathbf{A} = -\frac{1}{h^2}\begin{bmatrix} \mathbf{Q}_0 & \mathbf{Q}_0^+ & & & \\ \mathbf{Q}_1^- & \mathbf{Q}_1 & \mathbf{Q}_1^+ & & \\ & & \ddots & & \\ & & \mathbf{Q}_{\mathcal{I}-1}^- & \mathbf{Q}_{\mathcal{I}-1} & \mathbf{Q}_{\mathcal{I}-1}^+ \\ & & & \mathbf{Q}_{\mathcal{I}}^- & \mathbf{Q}_{\mathcal{I}} \end{bmatrix} \tag{SM4.9}$$

where

$$\begin{aligned} \mathbf{Q}_i^- &= \begin{bmatrix} (h/2)m_{i,0} - f_{i,0} & & & \\ & (h/2)m_{i,1} - f_{i,1} & & \\ & & \ddots & \\ & & & (h/2)m_{i,\mathcal{J}} - f_{i,\mathcal{J}} \end{bmatrix} \\ \mathbf{Q}_i^+ &= \begin{bmatrix} -(h/2)m_{i,0} - f_{i,0} & & & \\ & -(h/2)m_{i,1} - f_{i,1} & & \\ & & \ddots & \\ & & & -(h/2)m_{i,\mathcal{J}} - f_{i,\mathcal{J}} \end{bmatrix} \end{aligned} \tag{SM4.10}$$

and

(SM4.11)

$$\mathbf{Q}_i = \begin{bmatrix} 2f_{i,0} + \frac{h^2}{k^2}g_{i,0} & -\frac{h^2}{2k}n_{i,0} - \frac{h^2}{k^2}g_{i,0} & & & \\ \frac{h^2}{2k}n_{i,1} - \frac{h^2}{k^2}g_{i,1} & 2f_{i,1} + \frac{h^2}{k^2}g_{i,1} & -\frac{h^2}{2k}n_{i,1} - \frac{h^2}{k^2}g_{i,1} & & \\ & \frac{h^2}{2k}n_{i,2} - \frac{h^2}{k^2}g_{i,2} & 2f_{i,2} + \frac{h^2}{k^2}g_{i,2} & -\frac{h^2}{2k}n_{i,2} - \frac{h^2}{k^2}g_{i,2} & \\ & & \ddots & \ddots & \ddots \\ & & \frac{h^2}{2k}n_{i,\mathcal{J}-1} - \frac{h^2}{k^2}g_{i,\mathcal{J}-1} & 2f_{i,\mathcal{J}-1} + \frac{h^2}{k^2}g_{i,\mathcal{J}-1} & -\frac{h^2}{2k}n_{i,\mathcal{J}-1} - \frac{h^2}{k^2}g_{i,\mathcal{J}-1} \\ & & & \frac{h^2}{2k}n_{i,\mathcal{J}} - \frac{h^2}{k^2}g_{i,\mathcal{J}} & 2f_{i,\mathcal{J}} + \frac{h^2}{k^2}g_{i,\mathcal{J}} \end{bmatrix}$$

so that (SM4.7) may be written as a block linear system of the form

$$\mathbf{A}\mathbf{z} = \vec{0} \tag{SM4.12}$$

We now account for the vanishing Neumann boundary conditions by introducing so-called "ghost-nodes", which are subsequently eliminated by symmetry. This contribution is captured by two matrices, $\mathbf{L}_1$ and $\mathbf{L}_2$, introduced below.

First, consider boundary points $w_{0,j}$, and note that by (SM4.3) in conjunction with (SM4.6), we have that

$$\frac{-w_{-1,j} + w_{1,j}}{2h} = 0 \tag{SM4.13}$$

It follows that $w_{1,j} = w_{-1,j}$. Similarly, at boundary points $w_{\mathcal{I},j}$, we have that $w_{\mathcal{I}-1,j} = w_{\mathcal{I}+1,j}$. Consequently, the block matrix

$$\mathbf{L}_1 = -\frac{1}{h^2}\begin{bmatrix} \mathbf{0} & \mathbf{Q}_0^- & & \\ & & \ddots & \\ & & & \mathbf{Q}_{\mathcal{I}}^+ & \mathbf{0} \end{bmatrix} \tag{SM4.14}$$

eliminates the ghost nodes $w_{-1,j}$ and $w_{\mathcal{I}+1,j}$ by updating the $w_{1,j}$ and $w_{\mathcal{I}-1,j}$ coefficients. Now, by the same reasoning, boundary points of the form $w_{i,0}$ satisfy

$$\frac{-w_{i,-1} + w_{i,1}}{2k} = 0 \tag{SM4.15}$$

which implies that $w_{i,1} = w_{i,-1}$. Similarly, we find that $w_{i,\mathcal{J}-1} = w_{i,\mathcal{J}+1}$. Consequently, the matrix

(SM4.16)

$$\mathbf{L}_2 = -\frac{1}{h^2}\begin{bmatrix} \mathbf{T}_0 & & & \\ & \mathbf{T}_1 & & \\ & & \ddots & \\ & & & \mathbf{T}_{\mathcal{I}} \end{bmatrix}, \quad \mathbf{T}_i = \begin{bmatrix} 0 & \frac{h^2}{2k} n_{i,0} - \frac{h^2}{k^2} g_{i,0} & & \\ & & \ddots & \\ & & -\frac{h^2}{2k} n_{i,\mathcal{J}} - \frac{h^2}{k^2} g_{i,\mathcal{J}} & 0 \end{bmatrix}$$

eliminates the ghost nodes $w_{i,-1}$ and $w_{i,\mathcal{J}+1}$ by updating the $w_{i,1}$ and $w_{i,\mathcal{J}-1}$ coefficients. Let $\mathbf{L} = \mathbf{A} + \mathbf{L}_1 + \mathbf{L}_2$. Then, the system

$$\mathbf{L}\mathbf{z} = \vec{0} \tag{SM4.17}$$

discretizes the PDE (SM4.1). In the event that (SM4.1) corresponds to the backward equation for a stochastic oscillator, the eigenvalues and eigenvectors of $\mathbf{L}$ approximate the eigenvalues and eigenfunctions of the corresponding backward operator.

We recall that the forward operator, $\mathcal{L}$, and backward operator, $\mathcal{L}^\dagger$, are adjoint to each other (with appropriate boundary conditions). Consequently, $\mathbf{L}^T$ gives a discretization of the forward operator, and its eigenvectors approximate the eigenfunctions of $\mathcal{L}$.

## SM5. Further Examples.

In this section, we provide further details on examples considered in the main text. We also consider several other examples for the sake of completeness.

### SM5.1. 2D Noisy Stuart-Landau Oscillator.

Here, we recall the noisy 2D Stuart-Landau oscillator

$$\begin{aligned} dX &= [-4X(X^2 + Y^2 - 1) + \omega Y]dt + \sqrt{2D}\,dW_1(t) \\ dY &= [-4Y(X^2 + Y^2 - 1) - \omega X]dt + \sqrt{2D}\,dW_2(t) \end{aligned} \tag{SM5.1}$$

where we take $\omega = 2$ and $D = 0.09473$. We use finite differences to solve for the SKO and forward eigenpairs of (SM5.1), and treat the results as ground truth. For the ANN approach, we consider a numerical domain $\mathcal{R} = [-2, 2] \times [-2, 2]$ discretized into $N^2$ boxes, with $N = 200$. For reference, we list the first three leading SKO eigenvalues, as computed via finite differences

$$\lambda_1 = -0.1 + 2i, \quad \lambda_2 = -0.3988 + 4i, \quad \lambda_3 = -0.8931 + 6i \tag{SM5.2}$$

The real and imaginary parts of the first two forward and backward eigenfunctions are shown in Figures SM1 and SM2. Note that the stationary distribution, i.e., the eigenfunction $P_0$, is known exactly

$$P_0(x, y) = \frac{1}{N} \exp\left(-\frac{1}{D}(x^2 + y^2 - 1)^2\right), \quad N = \iint_{\mathbb{R}^2} dxdy \ \exp\left(-\frac{1}{D}(x^2 + y^2 - 1)^2\right) \tag{SM5.3}$$

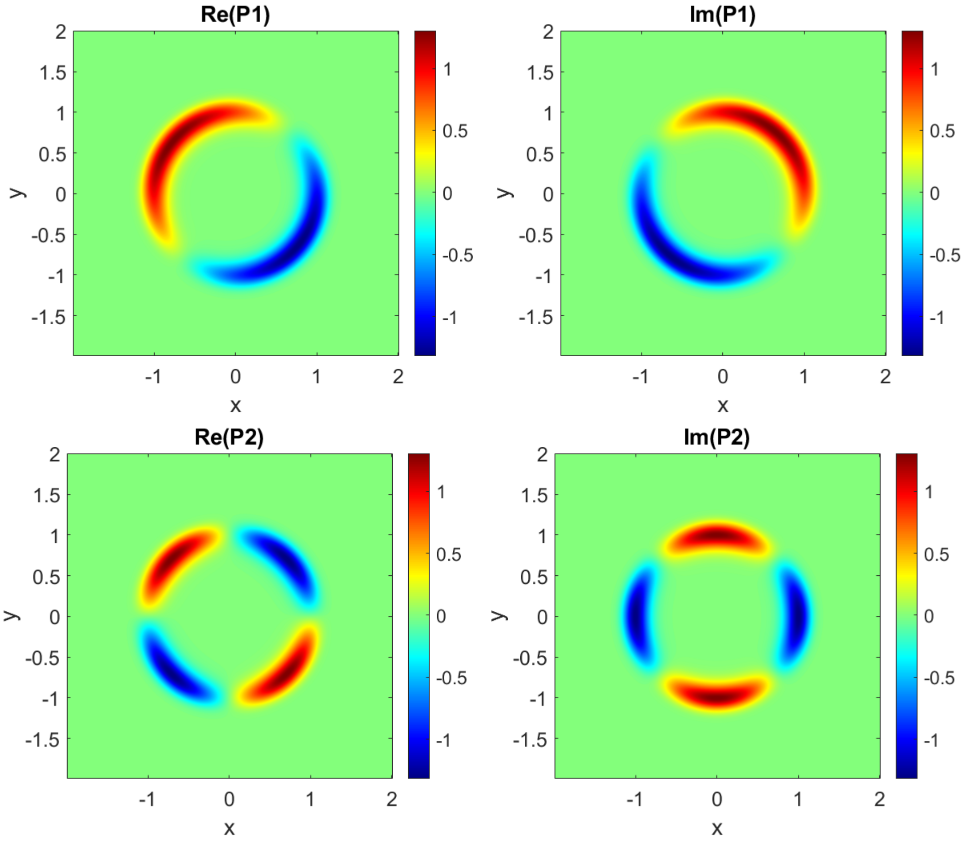


**Figure SM1.** *The low-lying FD forward eigenfunctions of the noisy 2D Stuart-Landau oscillator* (SM5.1). *The top row shows the real (left) and imaginary (right) parts of $P_{\lambda_1}$, and the bottom row shows the real (left) and imaginary (right) parts of $P_{\lambda_2}$.*

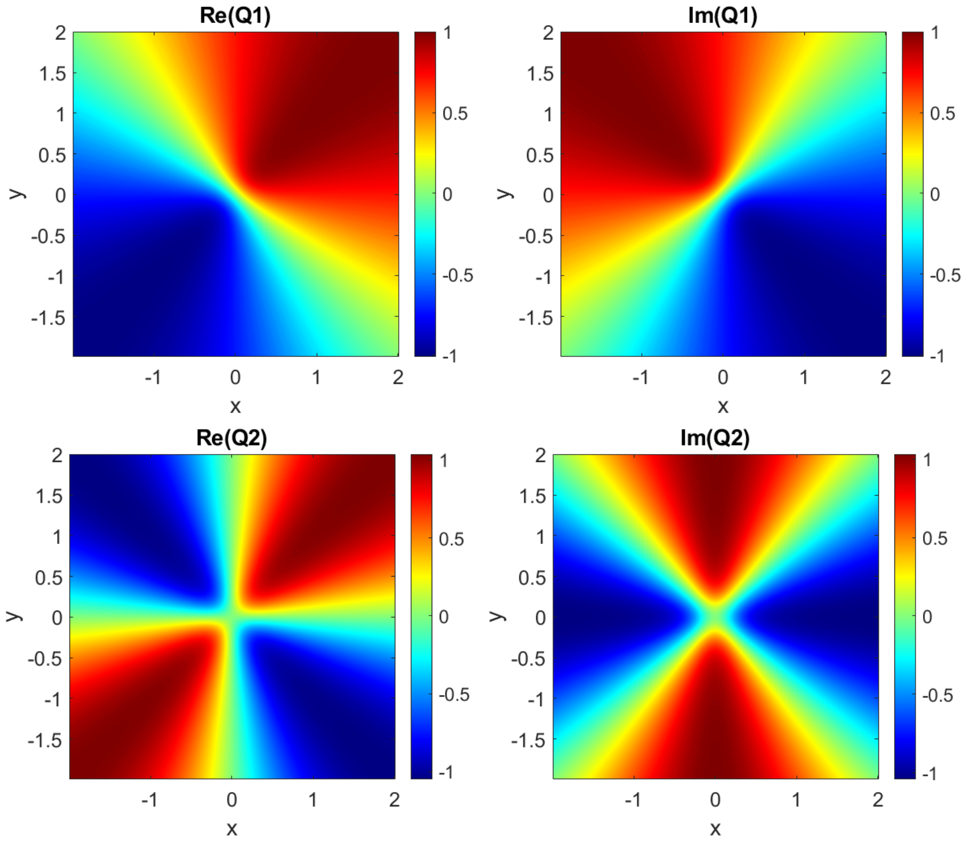


**Figure SM2.** *The low-lying FD backward eigenfunctions of the noisy 2D Stuart-Landau oscillator* (SM5.1). *The top row shows the real (left) and imaginary (right) parts of* $Q^*_{\lambda_1}$, *and the bottom row shows the real (left) and imaginary (right) parts of* $Q^*_{\lambda_2}$.

**SM5.1.1. Computation with one forward eigenmode.** We first consider the approximation of the forward eigenmode $P_{\lambda_1}$ using our ANN approach. We run 400,000 trajectories and sample the forward density at $N_t = 5000$ time-slices with timestep $dt = 0.001$ and $t_{\text{gap}} = 10$. Each realization has an initial condition drawn uniformly from the box containing the point $(1, 0)$. The reference box for the eigenvalue approximation is $\mathcal{B} = [-2, 0] \times [-2, 0]$.

In Figure SM3, we plot the decay of the forward time-dependent density in the reference box. The decaying density is fit to time-slices $t_k$ with $k \in [1000, 5000]$. Our fitting returns an estimated eigenvalue $\tilde{\lambda}_1 = -0.0996 + 2.0001i$. Both the real and imaginary parts have less than 1% relative error compared to the FD solution (see (SM5.2)).

In Figure SM4, we show the error results of the least squares approximation for the forward eigenfunctions including only one eigenmode in the computation. We choose the same time interval as for the eigenvalue approximation, $k \in [1000, 5000]$. The approximation is accurate[4], but is not very smooth. We display the output of the ANN, and report on the

[4]We normalize the FD and least squares eigenfunctions to have unit variance via [SM15], which fixes their magnitude. We utilize a gauge transformation [SM10] to fix the rotation of each eigenfunction, which allows

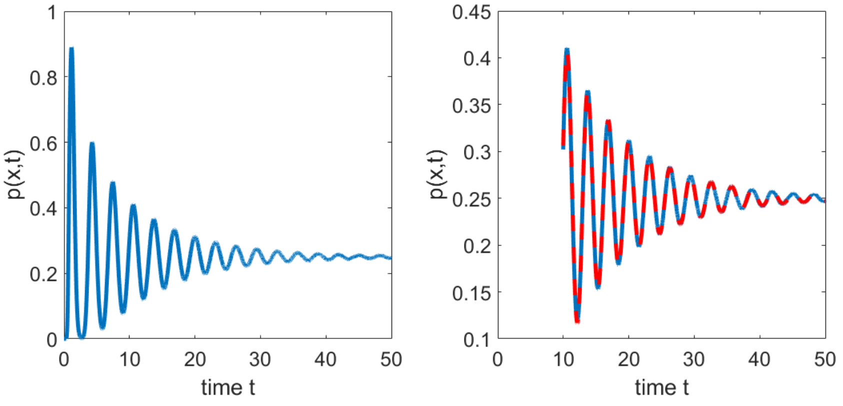


**Figure SM3.** *The decaying probability density (left) over $N_t = 5000$ time-slices for the 2D Stuart-Landau system* (SM5.1). *We fit the decaying density using only time-slices from $t_k$ for $k \in [1000, 5000]$ (red, right).*

discrete (relative) $L_2$ error[5]. We used $|\mathcal{Y}|$ =500,000 reference points, all 40,000 training points $\mathcal{X}$, and trained the ANN over 30 epochs. Iterations were broken up into 128 batches, which were optimized separately to improve speed. Results show that the ANN eigenfunctions are in good qualitative agreement with the true solution.

**SM5.1.2. Computation with three forward eigenmodes.** Note that with the eigenvalue approximation $\tilde{\lambda}_1 = -0.0996 + 2.0001i$, we may generate estimates of the higher-order eigenvalues by assuming that these low-lying eigenvalues lie on a parabola: $\lambda_n \approx -\mu_1 n^2 + i\omega_1 n$. Doing so gives the following approximations

$$\tilde{\lambda}_2 = -0.3986 + 4.0002i$$
$$\tilde{\lambda}_3 = -0.8968 + 6.0002i \tag{SM5.4}$$

which are in excellent agreement with the true values. We solve the least squares problem with $k \in [200, 5000]$ and include three low-lying eigenmodes in the objective function. We present error results for $P_{\lambda_1}$ in Figure SM5 and $P_{\lambda_2}$ in Figure SM6.

**SM5.1.3. Computation with three forward eigenmodes and few collocation points.** We now repeat the computation with three low-lying eigenmodes included in the least squares problem, but use only 5,000 (chosen randomly and uniformly) of the total 40,000 collocation points in $\mathcal{X}$ when training the ANN. Figure SM7 shows that the ANN output is similar to the previous case when all 40,000 boxes were used. The success of the ANN with relatively few collocation points allows for successful implementation in high dimensions, where it is computationally prohibitive to store large meshes.

for straightforward comparison.

[5]We define the relative $L_2$ error as $||u - \hat{u}||_{L_2}/||u||_{L_2}$ where $||u||_{L_2} = \sqrt{h_x h_y \sum_{i,j=1}^{N} |u_{i,j}|^2}$, Here, $u$ is the true solution, and $\hat{u}$ is an approximate solution. We assume uniform spacing $h_x$ and $h_y$ between gridpoints in the $x$ and $y$-coordinates, respectively.

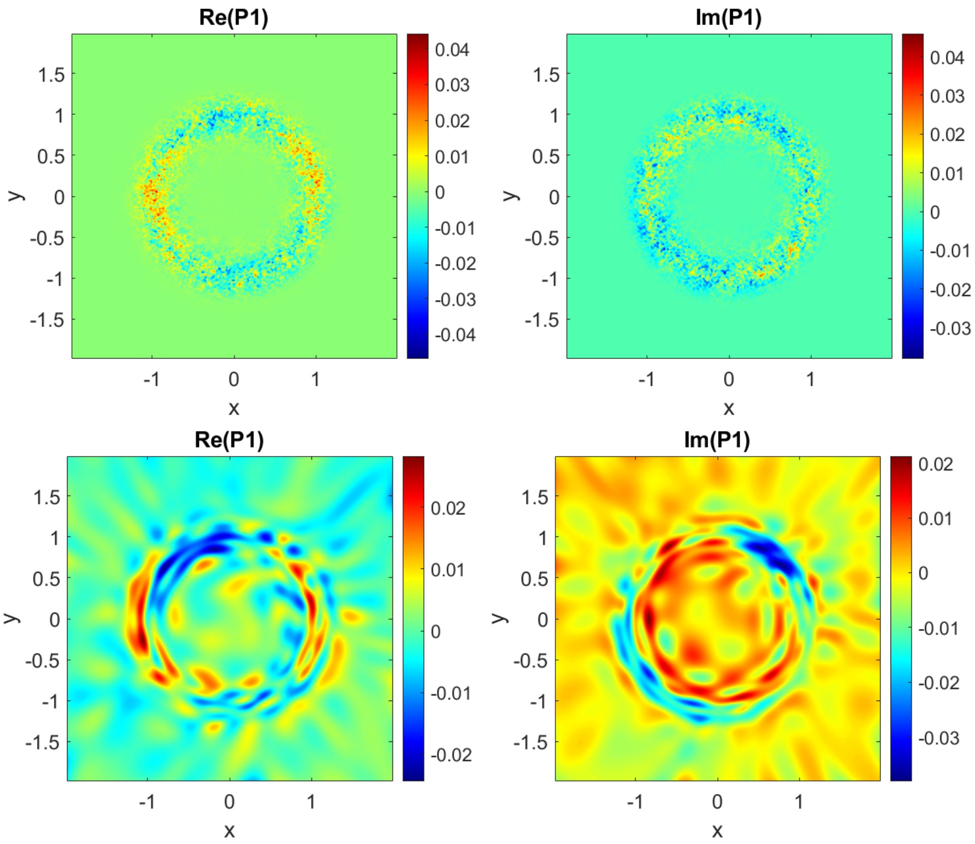


**Figure SM4.** *The error associated with* $P_{\lambda_1}$ *for the least squares fitting (top) and ANN solution (bottom). The* $L_2$ *error was computed to be* 0.0167 *and* 0.0218*, respectively.*

**SM5.1.4. Computation with one backward eigenmode.** We now repeat these experiments for the $Q$-function of the 2D Stuart-Landau model (SM5.1). We run 20,000 trajectories with initial conditions drawn uniformly on each of the $N^2 = 40{,}000$ boxes and sample the backward density at $N_t = 200$ time-slices with timestep $dt = 0.005$ and $t_{gap} = 20$. The reference box is $\mathcal{B} = [-2, 0] \times [-2, 0]$.

In Figure SM8, we plot the decay of (one of) the backward time-dependent densities in the reference box. The decaying density is fit to time-slices $t_k$ for $k \in [100, 200]$. Our fitting returns an estimate eigenvalue $\tilde{\lambda}_1 = -0.0992 + 1.9997i$. Once again, both the real and imaginary parts have less than 1% relative error compared to the FD solution (see equation (SM5.2)).

In Figure SM9, we display the error results of the least squares approximation for the forward and backward eigenfunctions including only one eigenmode in the computation. We choose a time interval, $k \in [70, 200]$. We also show the output of the ANN, and report on the discrete (relative) $L_2$ error. We used $|\mathcal{Y}|$ =500,000 reference points, all 40,000 training points $\mathcal{X}$, and trained the ANN over 30 epochs. Iterations were broken up into 128 batches, which were optimized separately to improve speed.

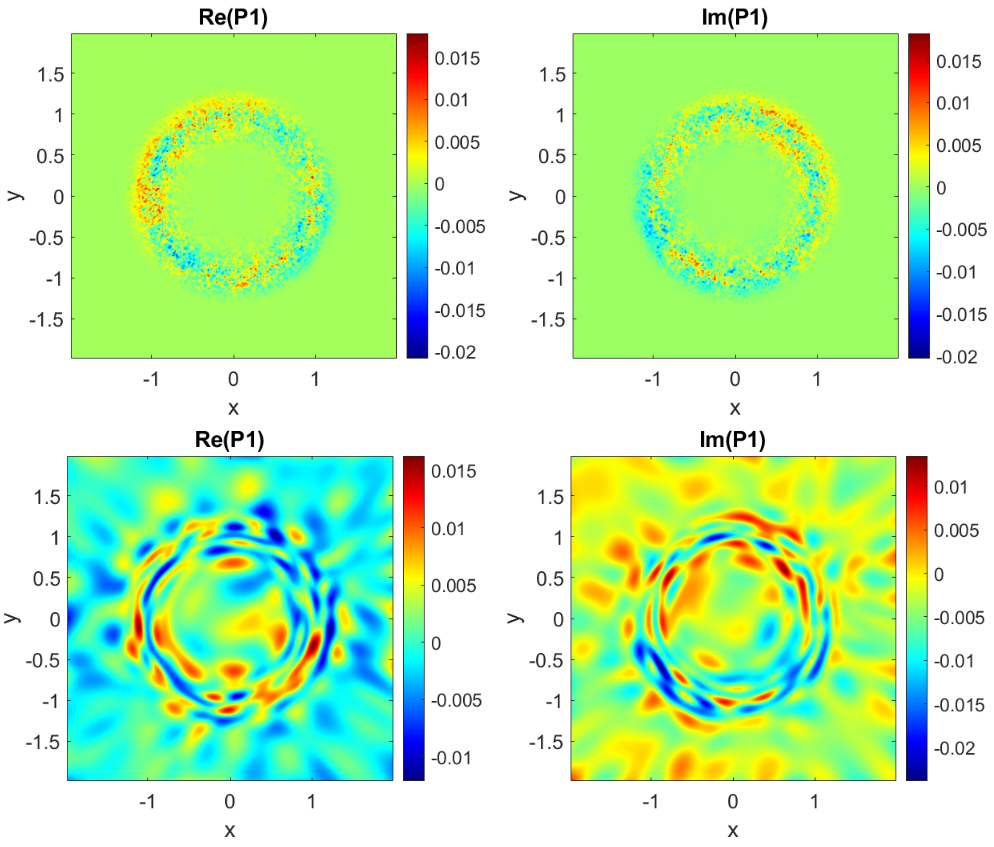


**Figure SM5.** *The error associated with $P_{\lambda_1}$ for the least squares fitting (top) and ANN solution (bottom) using three low-lying eigenmodes. In each case, the $L_2$ error was computed to be* 0.0079 *and* 0.0162*, respectively. Compare with Figure SM4.*

**SM5.1.5. Computation with three backward eigenmodes.** Note that with the eigenvalue approximation $\tilde{\lambda}_1 = -0.0992 + 1.99971i$, we may generate estimates of the higher-order eigenvalues by assuming (as in the forward case) that these low-lying eigenvalues lie on a parabola: $\lambda_n \approx -\mu_1 n^2 + i\omega_1 n$. Doing so gives

$$\begin{aligned}\tilde{\lambda}_2 &= -0.3970 + 3.9995i \\ \tilde{\lambda}_3 &= -0.8932 + 5.9992i\end{aligned} \qquad \text{(SM5.5)}$$

which are in excellent agreement with the true values, see equation (SM5.2). We solve the least squares problem with $k \in [20, 200]$ and include three low-lying eigenmodes in the objective function. We present error results for $Q^*_{\lambda_1}$ in Figure SM10 and $Q^*_{\lambda_2}$ in Figure SM11.

**SM5.1.6. Computation with three backward eigenmodes and few collocation points.** We now repeat the computation with three low-lying eigenmodes included in the least squares problem, but use only 5,000 (chosen randomly and uniformly) of the total 40,000 collocation points in $\mathcal{X}$ when training the ANN. Figure SM12 shows that the ANN output is similar to the previous case when all 40,000 boxes were used. We emphasize again that the success of

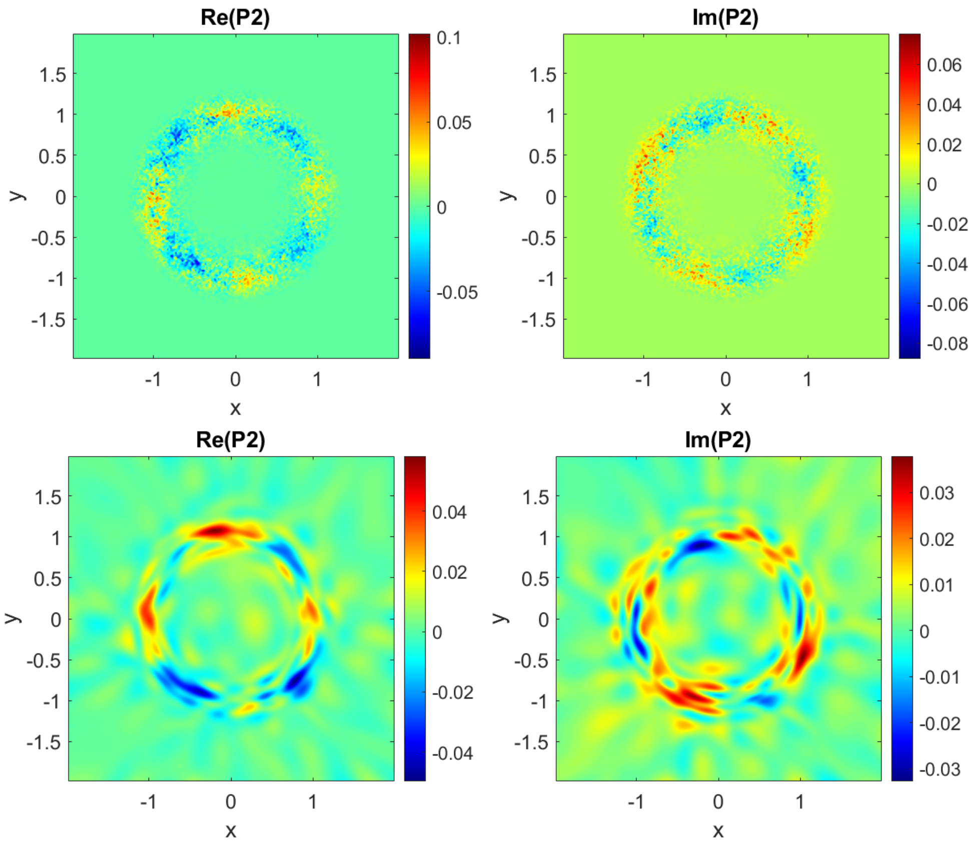


**Figure SM6.** *The error associated with* $P_{\lambda_2}$ *for the least squares fitting (top) and ANN solution (bottom) using three low-lying eigenmodes. In each case, the* $L_2$ *error was computed to be* 0.0339 *and* 0.0269*, respectively.*

the ANN with relatively few collocation points allows for a successful implementation in high dimensions, where it is computationally prohibitive to store large meshes.

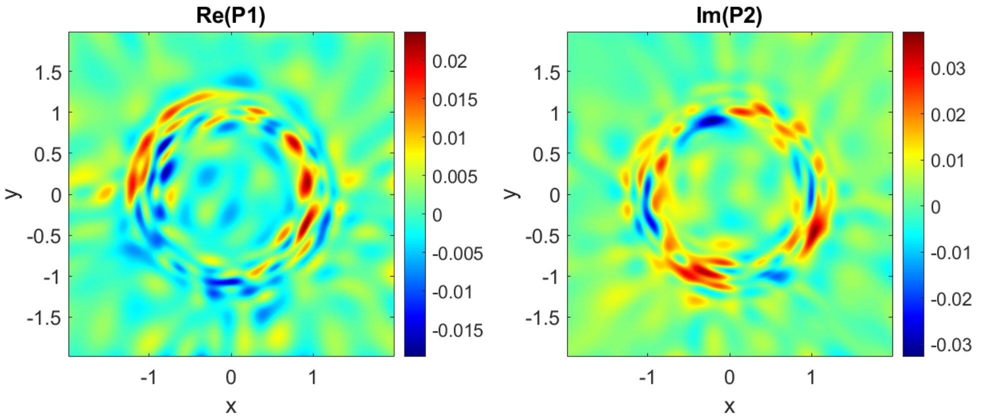


**Figure SM7.** *The error associated with* $P_{\lambda_1}$ *for the ANN solution using three low-lying eigenmodes but only 5,000 collocation points. The* $L_2$ *error was computed to be* 0.0151*. Results should be compared with the bottom row of Figure SM5.*

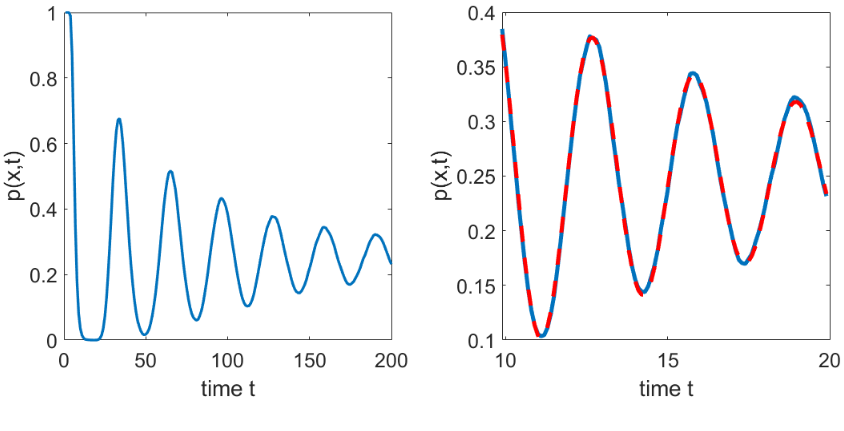


**Figure SM8.** *The decaying probability density (left) over* $N_t = 200$ *time-slices for the 2D Stuart-Landau system* (SM5.1)*. We fit the decaying density using only timeslices from* $t_k$ *for* $k \in [100, 200]$ *(red, right).*

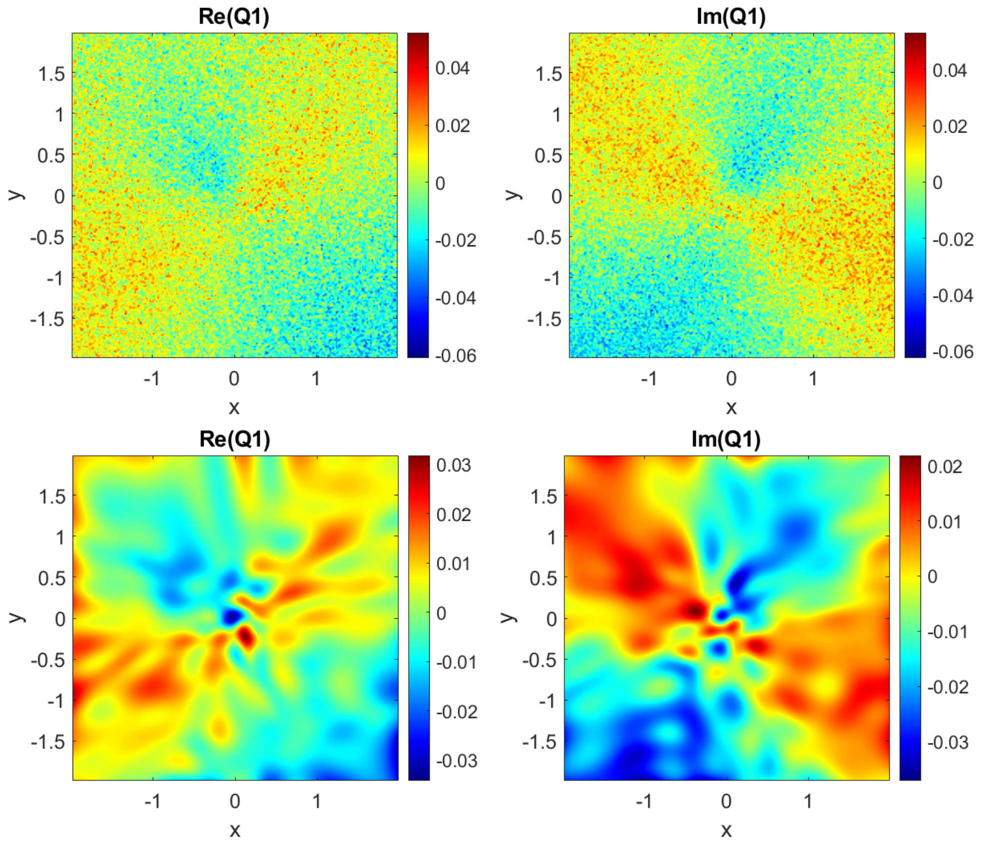


**Figure SM9.** *The error associated with $Q^*_{\lambda_1}$ for the least squares fitting (top) and ANN solution (bottom). The $L_2$ error was computed to be 0.0210 and 0.0156, respectively.*

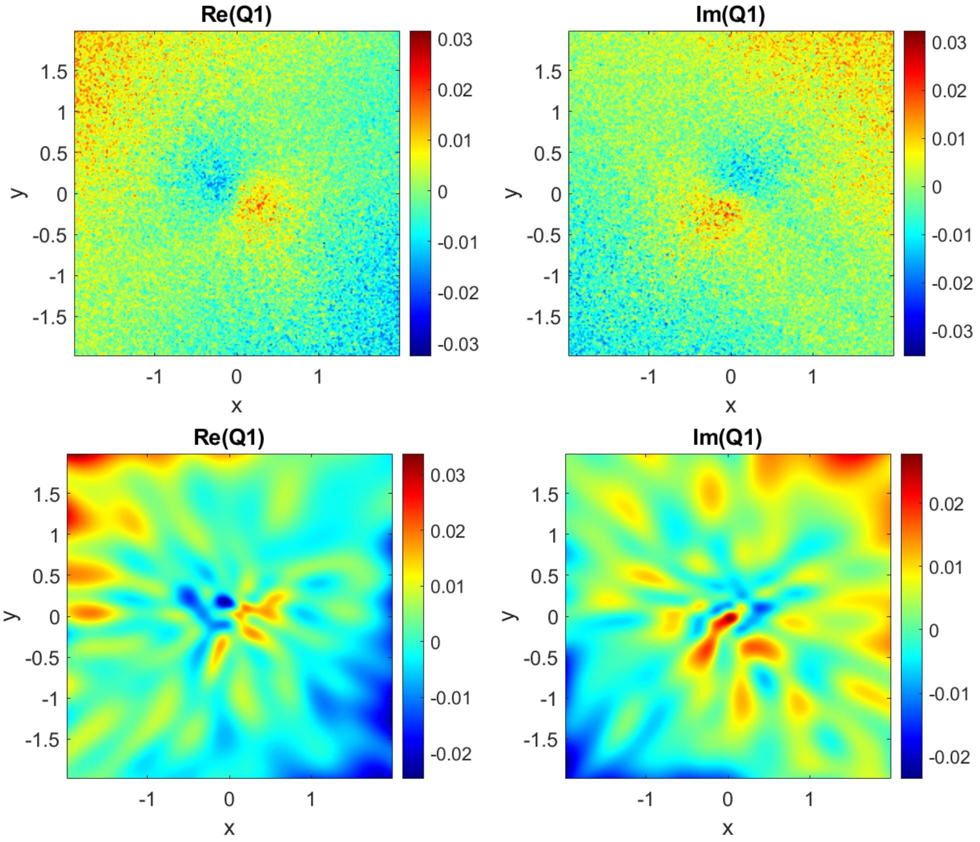


**Figure SM10.** *The error associated with* $Q^*_{\lambda_1}$ *for the least squares fitting (top) and ANN solution (bottom) using three low-lying eigenmodes. In each case, the* $L_2$ *error was computed to be* 0.0103 *and* 0.0095*, respectively. Compare with Figure SM9.*

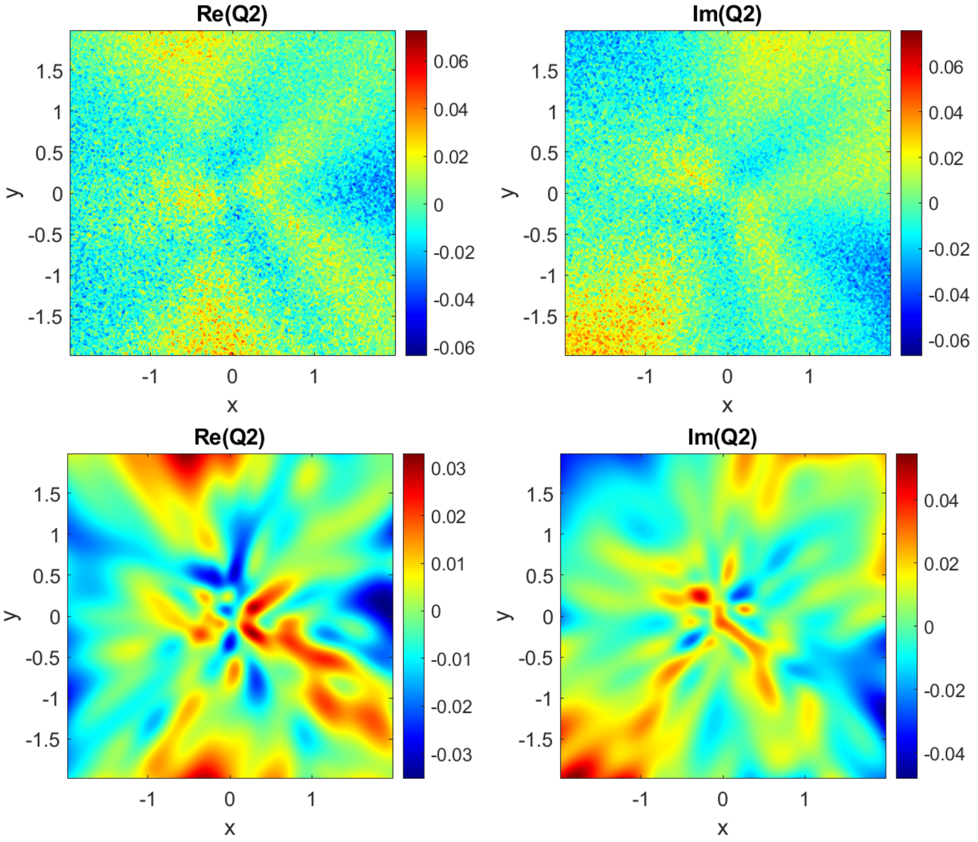


**Figure SM11.** *The error associated with* $Q^*_{\lambda_2}$ *for the least squares fitting (top) and ANN solution (bottom) using three low-lying eigenmodes. In each case, the* $L_2$ *error was computed to be* 0.0220 *and* 0.0166*, respectively.*

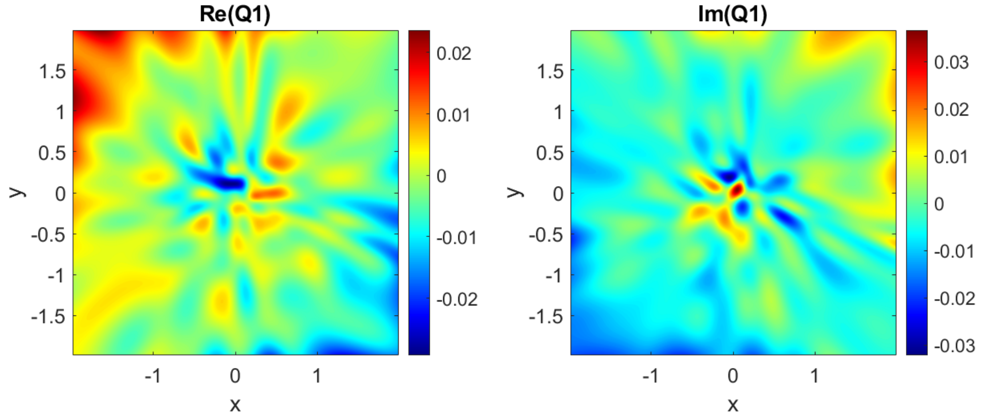


**Figure SM12.** *The error associated with* $Q^*_{\lambda_1}$ *for the ANN solution using three low-lying eigenmodes but only 5,000 collocation points. The* $L_2$ *error was computed to be* 0.0091*. Results should be compared with the bottom row of Figure SM10.*

**SM5.2. 2D Morris-Lecar Neuron.** In this section, we consider a 2D Morris-Lecar neuron with multiplicative channel noise and additive current noise

$$dV = \frac{\iota}{C}\left[I - g_L(V - v_L) - g_K N(V - v_K) - g_{CA} m_\infty(V)(V - v_{CA})\right] dt + \sqrt{2D_v}\, dW_1(t)$$
$$dN = \iota\left[\alpha(V)(1-N) - \beta(V)N\right] dt + \epsilon\sqrt{\alpha(V)(1-N) + \beta(V)N}\, dW_2(t) \tag{SM5.6}$$

where functions and parameter values for the noiseless system are as in section SM6, and $\iota = 20$ is introduced to increase the mean frequency of oscillation so that the leading SKO eigenvalues are on the same order of magnitude as for the 2D Stuart-Landau system considered above. The noise parameters are $\epsilon = 0.5$ and $D_v = 25$.

We use finite differences to solve for the backward eigenfunctions of (SM5.6), and treat the results as ground truth. For our ANN implementation, we consider a numerical domain $\mathcal{R} = [-90, 90] \times [0, 1]$ discretized into $N^2$ boxes, with $N = 200$. For reference, we list the first three leading SKO eigenvalues, as computed via finite differences

$$\lambda_1 = -0.1748 + 1.9597i, \quad \lambda_2 = -0.4953 + 4.0437i, \quad \lambda_3 = -0.9512 + 6.1771i \tag{SM5.7}$$

The stationary distribution is shown in Figure SM13. The real and imaginary parts of the leading backward eigenfunctions are shown in Figure SM14.

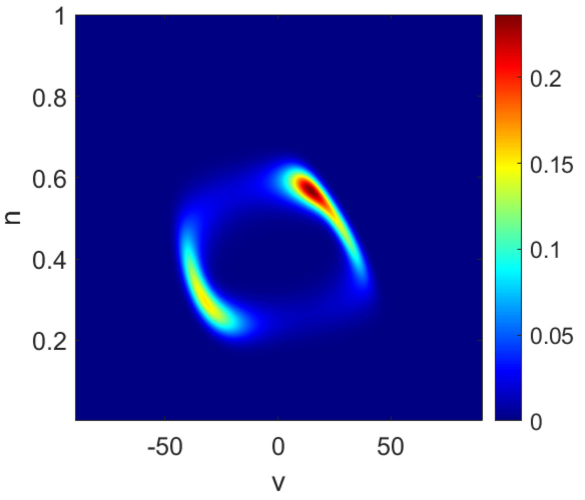


**Figure SM13.** *The stationary distribution for the 2D Morris-Lecar model* (SM5.6).

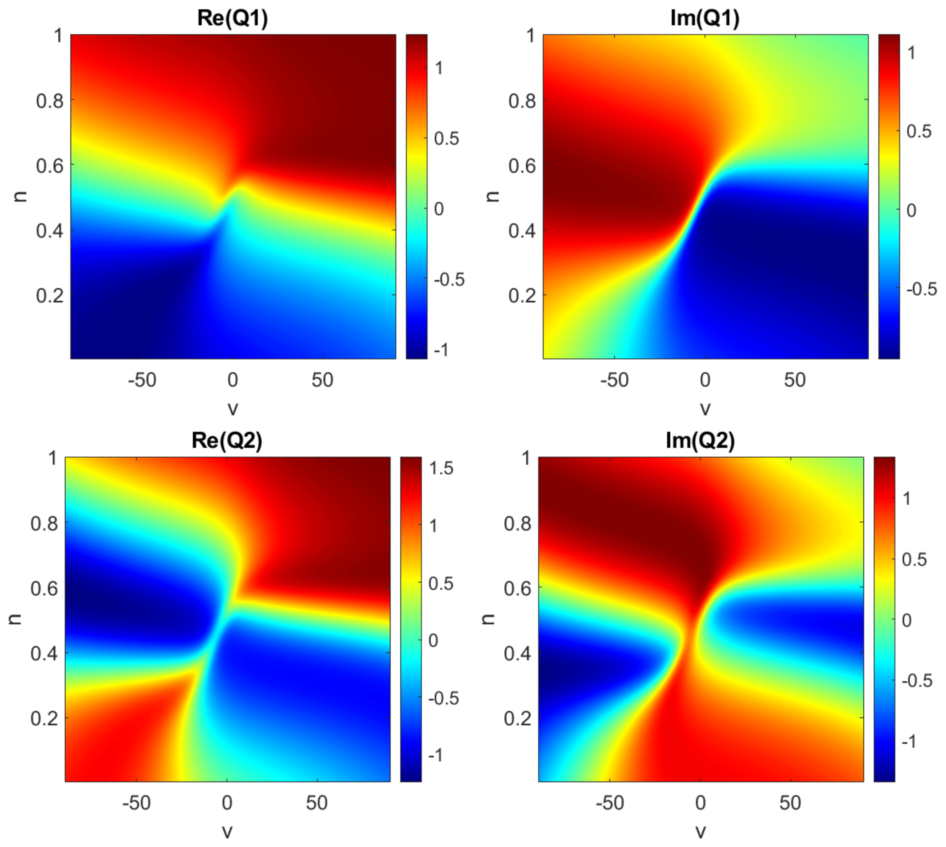


**Figure SM14.** *The low-lying backward eigenfunctions of the noisy 2D Morris-Lecar neuron* (SM5.6). *The top row shows the real (left) and imaginary (right) parts of* $Q^*_{\lambda_1}$, *and the bottom row shows the real (left) and imaginary (right) parts of* $Q^*_{\lambda_2}$.

We use our ANN approach to approximate $Q^*_{\lambda_1}$ and $Q^*_{\lambda_2}$ corresponding to the 2D Morris-Lecar model (SM5.6). We run 20,000 trajectories with initial conditions drawn uniformly on each of the $N^2 = 40,000$ boxes and sample the backward density at $N_t = 200$ time-slices with timestep $dt = 0.005$ and $t_{\text{gap}} = 20$. The reference box is $\mathcal{B} = [0, 90] \times [0.5, 1]$.

In Figure SM15, we plot the decay of (one of) the backward time-dependent densities in the reference box. The decaying density is fit to time-slices $t_k$ for $k \in [85, 200]$. Our fitting returns an estimate eigenvalue $\tilde{\lambda}_1 = -0.1773 + 1.9565i$. Once again, both the real and imaginary parts have roughly 1% relative error compared to the FD solution (see equation (SM5.7)).

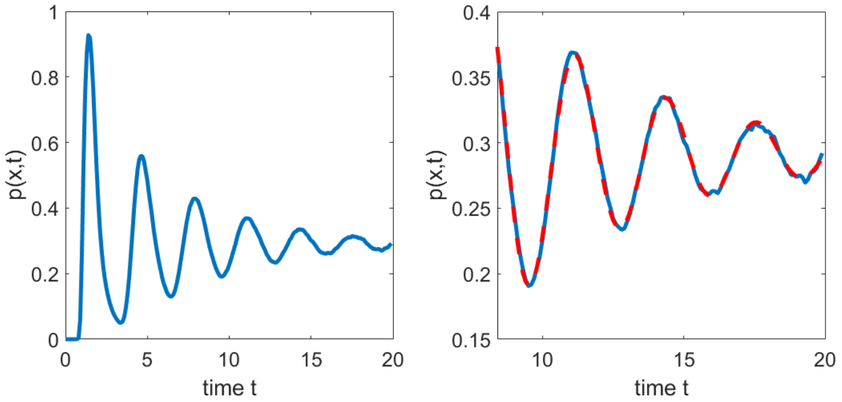


**Figure SM15.** *The decaying probability density (left) over $N_t = 200$ time-slices for the 2D Morris-Lecar system* (SM5.6). *We fit the decaying density using only timeslices from $t_k$ for $k \in [85, 200]$ (red, right).*

In Figure SM16, we plot the error results for $Q^*_{\lambda_1}$. Error results for $Q^*_{\lambda_2}$ are shown in Figure SM17. We use (SM5.7) for the eigenvalue approximations. We choose a time interval, $k \in [10, 200]$. We display the output of the ANN, and report on the discrete $L_2$ error. We used $|\mathcal{Y}|$ =500,000 reference points, all 40,000 training points $\mathcal{X}$, and trained the ANN over 30 epochs. Iterations were broken up into 64 batches, which were optimized separately to improve speed. The hidden layers each consist of 350 nodes.

The 2D Morris-Lecar model has state variables which have different orders of magnitude, which can cause the ANN approximation to worsen. Therefore, when training the ANN, we rescale voltage $\overline{v} = V/100$ to be on the same order of magnitude as the gating variable $N$. Note that the first and second voltage derivatives in the backward equation should be rescaled accordingly. We display output using the unscaled coordinates.

**SM5.3. Commentary on the 2D examples.** We remark that the Monte Carlo approximation of the eigenfunctions tends to exhibit relative error on the order of $10^{-2}$ or $10^{-3}$. In part, this error is due to contamination from higher-order eigenmodes which results in spatially correlated errors in our least squares approximation, which the ANN struggles to overcome[6]. We find that including high-order modes in our least squares objective function

[6]In [SM20], the authors show that the ANN setup is adept at ameliorating errors that arise from spatially uncorrelated errors when approximating high-dimensional stationary distributions.

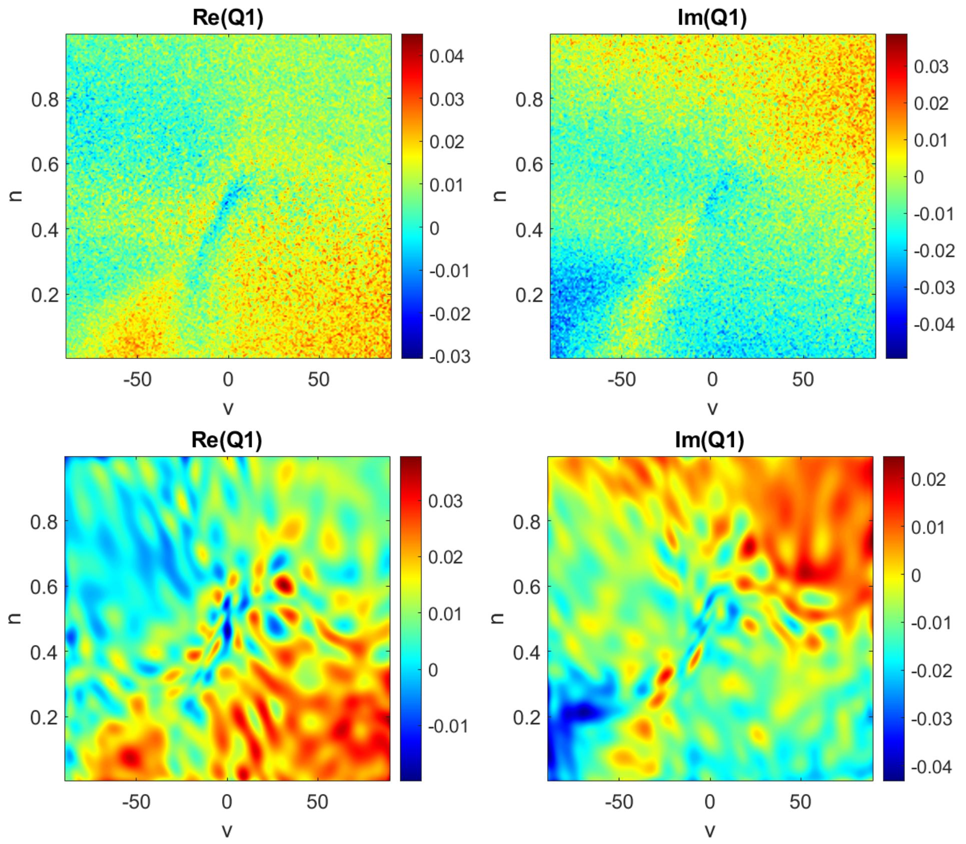


**Figure SM16.** *The error associated with* $Q^*_{\lambda_1}$ *for the least squares fitting (top) and ANN solution (bottom) using three low-lying eigenmodes. In each case, the* $L_2$ *error was computed to be* 0.0160 *and* 0.0165*, respectively.*

improves accuracy, but that some error remains. Regardless, the ANN retains accuracy even when relatively few collocation points are available for training. This property positions our ANN approach for success in higher-dimensional systems.

**SM5.4. 4D Noisy Coupled Staurt-Landau Oscillators.** Here, we study a system of coupled noisy Stuart-Landau oscillators

$$
\begin{aligned}
x_1' &= -4x_1(x_1^2 + x_2^2 - 1) + (\omega + \tau)x_2 + \kappa(y_1 - x_1) + \sqrt{2D_1}\xi_1(t) \\
x_2' &= -4x_2(x_1^2 + x_2^2 - 1) - (\omega + \tau)x_1 + \kappa(y_2 - x_2) + \sqrt{2D_1}\xi_2(t) \\
y_1' &= -4y_1(y_1^2 + y_2^2 - 1) + \omega y_2 + \kappa(x_1 - y_1) + \sqrt{2D_2}\xi_3(t) \\
y_2' &= -4y_2(y_1^2 + y_2^2 - 1) - \omega y_1 + \kappa(x_2 - y_2) + \sqrt{2D_2}\xi_4(t)
\end{aligned}
\tag{SM5.8}
$$

where $\omega = 2$, $\tau = 0.5$, $D_1 = 0.6$, and $D_2 = 0.09473$. The 2D example indicates that the effects of higher-order eigenmodes can influence the accuracy of our least squares approximation. Therefore, we increase the noise of the first oscillator so that its isolated eigenvalues have more negative real parts, i.e., so that the dominant SKO eigenvalues of (SM5.8) correspond only to the second oscillator (which are listed in equation (SM5.2)). Here, we set $\kappa = 0$ so

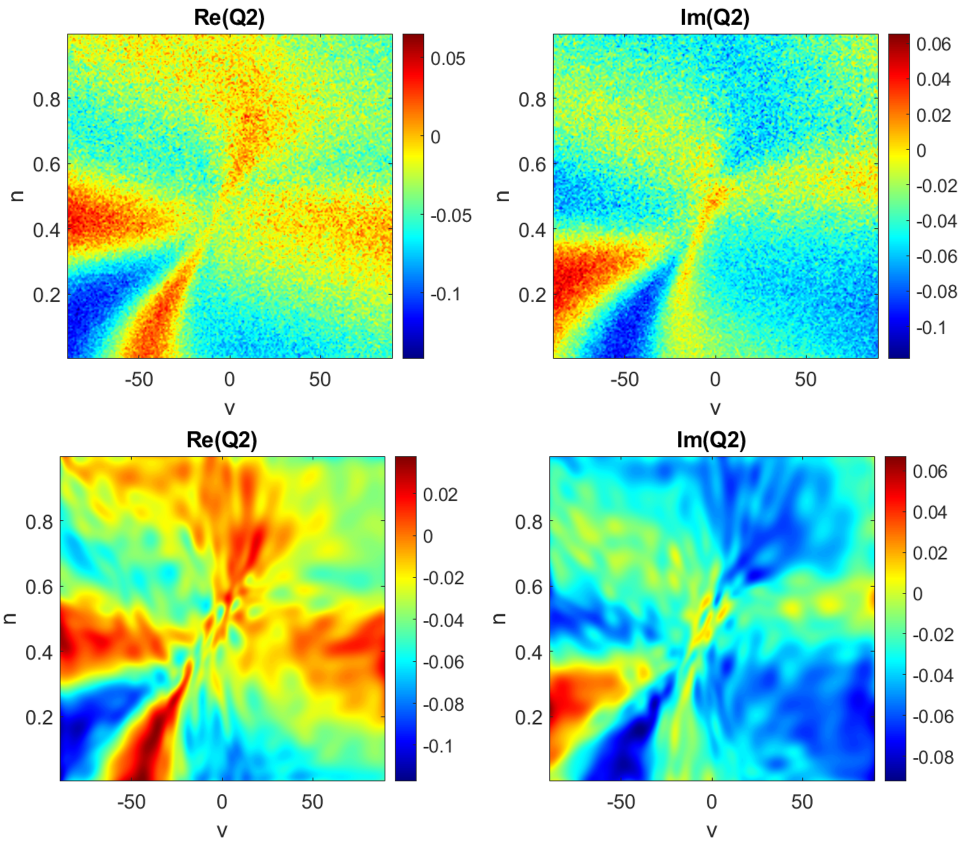


**Figure SM17.** *The error associated with $Q^*_{\tilde{\lambda}_2}$ for the least squares fitting (top) and ANN solution (bottom) using three low-lying eigenmodes. In each case, the $L_2$ error was computed to be* 0.0484 *and* 0.0440*, respectively.*

that the oscillators are uncoupled, i.e., so that we can project a 4D solution onto a 2D plane and compare with known solutions generated by finite differences.

To generate densities, we formally discretize the domain $\mathcal{R} = [-2, 2]^4$ into $N^4$ boxes, with $N = 100$. We store only 10,000 of the boxes in memory, chosen uniformly throughout $\mathcal{R}$. We take 20,000 initial conditions in each box, and keep track of the corresponding densities at $N_t = 300$ time-slices. We set $t_{\text{gap}} = 20$ and $dt = 0.005$. In Figure SM18, we depict the decaying probability density corresponding to one of the boxes. Our fitting procedure estimates that $\tilde{\lambda}_1 = -0.1001 + 1.9993i$ taking time-slices $t_k$ with $k \in [35, 300]$, which is in excellent agreement with the true value, $\lambda_1 = -0.1 + 2i$.

To generate approximations of the $Q$-function, we solve the least squares problem, and include the first three non-trivial eigenmodes in the expansion. As before, we may use the approximated eigenvalue $\tilde{\lambda}_1$ to generate approximations to the higher-order eigenvalues $\tilde{\lambda}_2$ and $\tilde{\lambda}_3$. We solve only with time-slices $t_k$ for $k \in [35, 200]$. Once this data is generated, we train an ANN on the 10,000 collocation points $\mathcal{X}$, and $|\mathcal{Y}|$ =1,000,000 reference points. The ANN was trained over 300 epochs, and iterations were divided into 128 batches, which were optimized separately to improve speed. In this case, the hidden layers of the ANN consist of

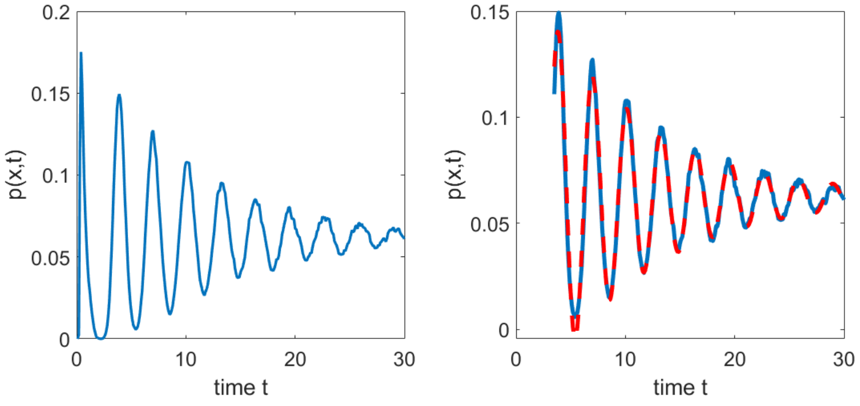


**Figure SM18.** *The decaying probability density (left) over $N_t = 300$ time-slices for the 4D Stuart-Landau system* (SM5.8)*. We fit the decaying density using only timeslices from $t_k$ for $k \in [35, 300]$ (red, right).*

only 20 nodes.

To gauge the accuracy of the least squares procedure and the ANN output, we used a finite difference method to compute the $Q$-function for the second isolated $(y_1, y_2)$ oscillator in (SM5.8) on a fine $400 \times 400$ mesh. Then, these finite-difference (FD) values were interpolated onto the 10,000 collocation points $\mathcal{X}$, so that a direct comparison could be made with the least squares output. While we train the ANN on only the collocation points $\mathcal{X}$, we evaluate the trained ANN on the fine FD mesh. We also trained the ANN on the interpolated FD points (as opposed to the least squares approximations at those points). We produce plots of two-dimensional projections of the $Q$-function for the least squares and ANN solutions in Figure SM19. The error results are shown in Figure SM20.

**SM5.5. 4D Noisy Coupled Morris-Lecar Neurons.** Here, we study a system of two noisy Morris-Lecar neurons coupled by a gap junction

$$
\begin{aligned}
dV_1 &= \frac{\iota}{C}[I - g_L(V_1 - v_L) - g_K N_1(V_1 - v_K) - g_{CA} m_\infty(V_1)(V_1 - v_{CA}) \\
&\quad + \kappa(V_2 - V_1)]dt + \sqrt{2D_{v_1}}\, dW_1(t) \\
dN_1 &= \iota\,[\alpha(V_1)(1 - N_1) - \beta(V_1)N_1]\, dt + \epsilon_1 \sqrt{\alpha(V_1)(1 - N_1) + \beta(V_1)N_1}\, dW_2(t) \\
dV_2 &= \frac{\iota}{C}[I - g_L(V_2 - v_L) - g_K N_2(V_2 - v_K) - g_{CA} m_\infty(V_2)(V_2 - v_{CA}) \\
&\quad + \kappa(V_1 - V_2)]dt + \sqrt{2D_{v_2}}\, dW_3(t) \\
dN_2 &= \iota\,[\alpha(V_2)(1 - N_2) - \beta(V_2)N_2]\, dt + \epsilon_2 \sqrt{\alpha(V_2)(1 - N_2) + \beta(V_2)N_2}\, dW_4(t)
\end{aligned}
\tag{SM5.9}
$$

where functions and parameter values for the noiseless system are as in section SM6, and $\iota = 20$. The noise parameters are $D_{v_1} = 15$, $D_{v_2} = 50$, $\epsilon_1 = 0.3$, and $\epsilon_2 = 1$. The 2D example indicates that pollution from higher-order eigenmodes can influence the accuracy of our least squares approximation. Therefore, we increase the noise of the second oscillator so that its isolated eigenvalues have more negative real parts, i.e., so that the dominant SKO eigenvalues of (SM5.9) correspond only to the first oscillator. Here, we set $\kappa = 0$ so that the oscillators are

uncoupled, i.e., so that we can project a 4D solution onto a 2D plane and compare with known solutions generated by finite differences. For reference, the first two eigenvalues (computed with finite-differences) are

$$\lambda_1 = -0.0879 + 1.9518i, \quad \lambda_2 = -0.2521 + 3.9602i \tag{SM5.10}$$

To generate densities, we formally discretize the domain $\mathcal{R} = [-90, 90] \times [0, 1] \times [-90, 90] \times [0, 1]$ into $N^4$ boxes, with $N = 100$. We store only 10,000 of the boxes in memory, chosen randomly and uniformly throughout $\mathcal{R}$. We take 30,000 initial conditions in each box, and keep track of the corresponding densities at $N_t = 350$ time-slices. We set $t_{\text{gap}} = 20$ and $dt = 0.005$. In Figure SM21, we depict the decaying probability density corresponding to one of the boxes. Our fitting procedure estimates that $\tilde{\lambda}_1 = -0.0871 + 1.9573i$ taking time-slices $t_k$ with $k \in [125, 350]$, which is in excellent agreement with the true value (see (SM5.10)).

To generate approximations of the $Q$-function, we solve the least squares problem and include the first two non-trivial eigenmodes in the expansion. We use (SM5.10) for the eigenvalue approximations. We solve only with time-slices $t_k$ for $k \in [125, 350]$. Once this data is generated, we train an ANN on the 10,000 collocation points $\mathcal{X}$, and $|\mathcal{Y}|$ =1,000,000 reference points. The ANN was trained over 200 epochs, and iterations were divided into 128 batches, which were optimized separately to improve speed. In this case, the hidden layers of the ANN consist of only 12 nodes. As in the 2D case, in our ANN implementation we rescale voltage $\overline{v_j} = V_j/100$ for $j = 1, 2$ to be on the same order of magnitude as the gating variables $N_j$.

To gauge the accuracy of the least squares procedure and the ANN output, we used a finite difference method to compute the $Q$-function for the first isolated $(V_1, N_1)$ oscillator in (SM5.9) on a fine $400 \times 400$ mesh. Then, these finite-difference (FD) values were interpolated onto the 10,000 collocation points $\mathcal{X}$, so that a direct comparison could be made with the least squares output. While we train the ANN on only the collocation points $\mathcal{X}$, we evaluate the trained ANN on the fine FD mesh. We produce plots of two-dimensional projections of the $Q$-function for the least squares and ANN solutions in Figure SM22. The error results are shown in Figure SM23.

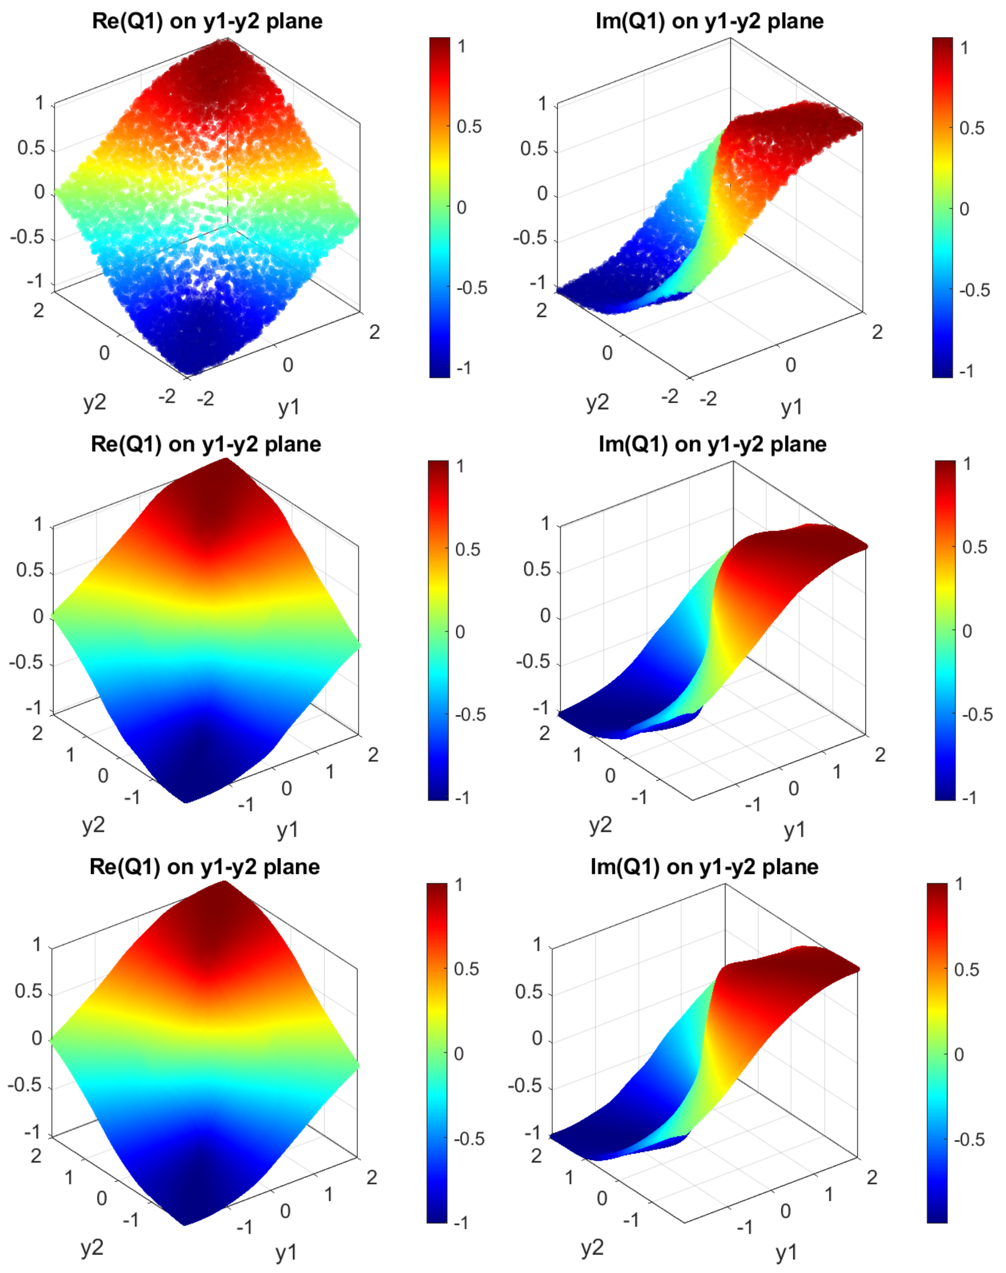


**Figure SM19.** *A projection of the 4D Q-function of* (SM5.8) *onto the* $(y_1, y_2)$*-plane with* $x_1 = 0$ *and* $x_2 = 0$*.* ***Top row:*** *the least squares approximation at the 10,000 collocation points* $\mathcal{X}$*.* ***Middle row:*** *the output of the ANN on a fine mesh, trained at the points* $\mathcal{X}$ *using the least squares values.* ***Bottom row:*** *the output of the ANN on a fine mesh, trained at the points* $\mathcal{X}$ *using the "true" finite difference values.*

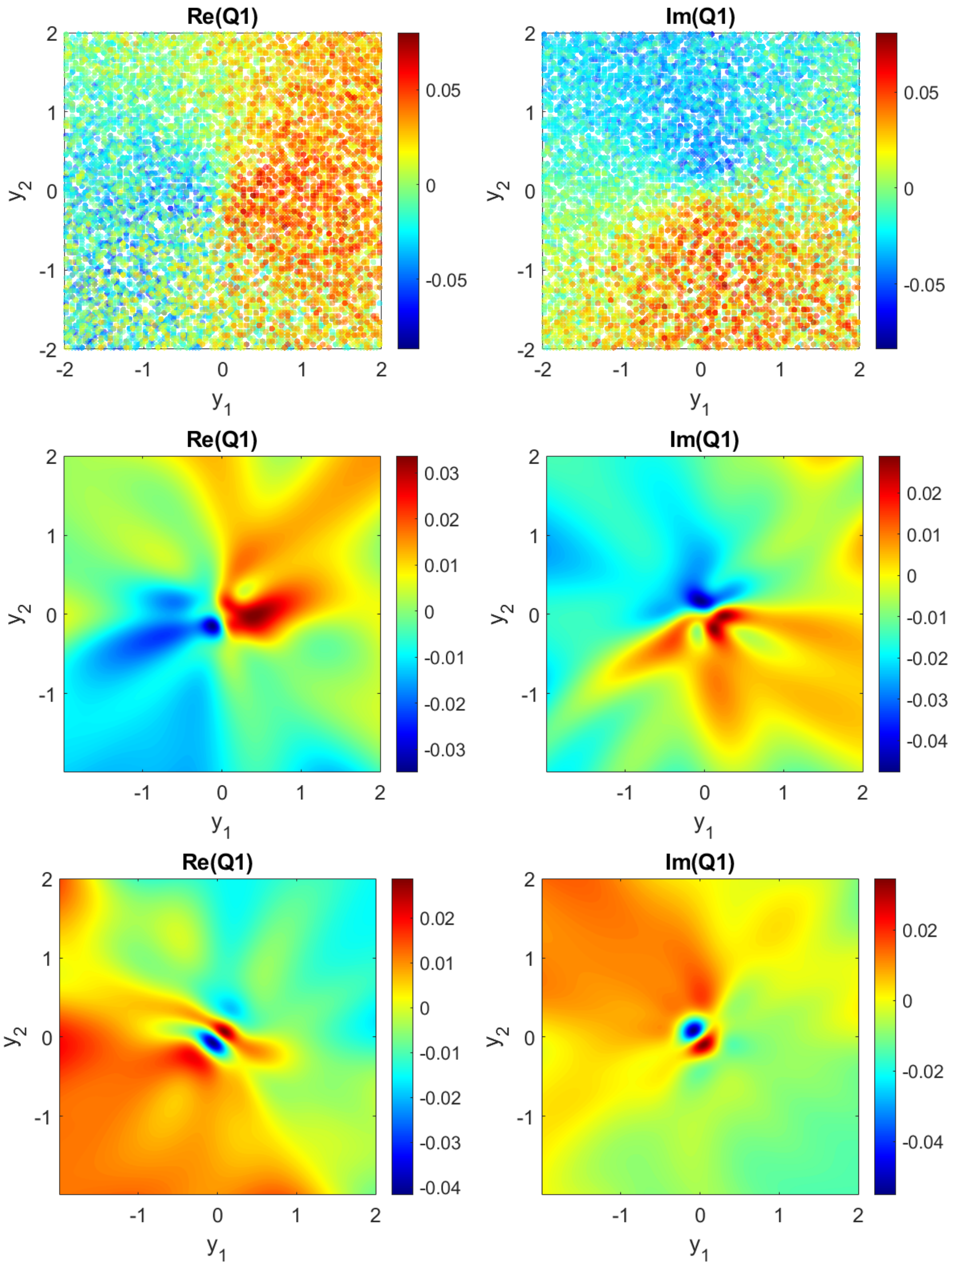


**Figure SM20.** *Heat maps of the error associated with the approximations of the 4D Q-function shown in Figure SM19.* ***Top row:*** *Difference of the least squares output and FD output at the collocation points* $\mathcal{X}$. ***Middle row:*** *Difference of the ANN output trained with the least squares data and the FD output on a fine mesh. The* $L_2$ *error is* 0.0159. ***Bottom row:*** *Difference of the ANN output trained with the FD data and the FD output on a fine mesh. The* $L_2$ *error is* 0.0126.

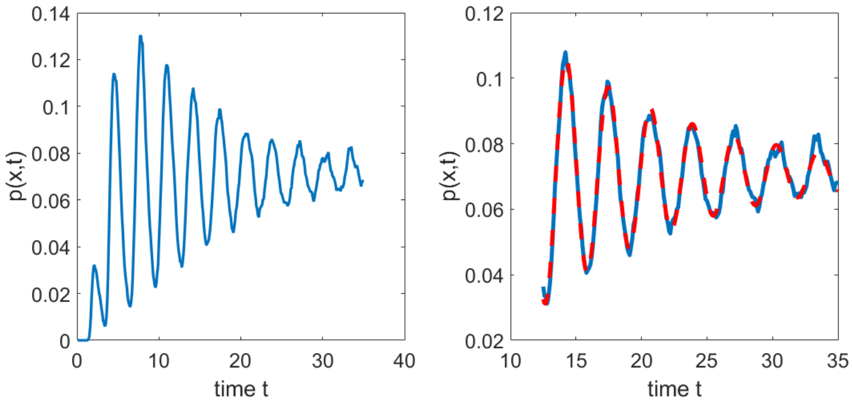


**Figure SM21.** *The decaying probability density (left) over $N_t = 350$ time-slices for the 4D Morris-Lecar system (SM5.9). We fit the decaying density using only timeslices from $t_k$ for $k \in [125, 350]$ (red, right).*

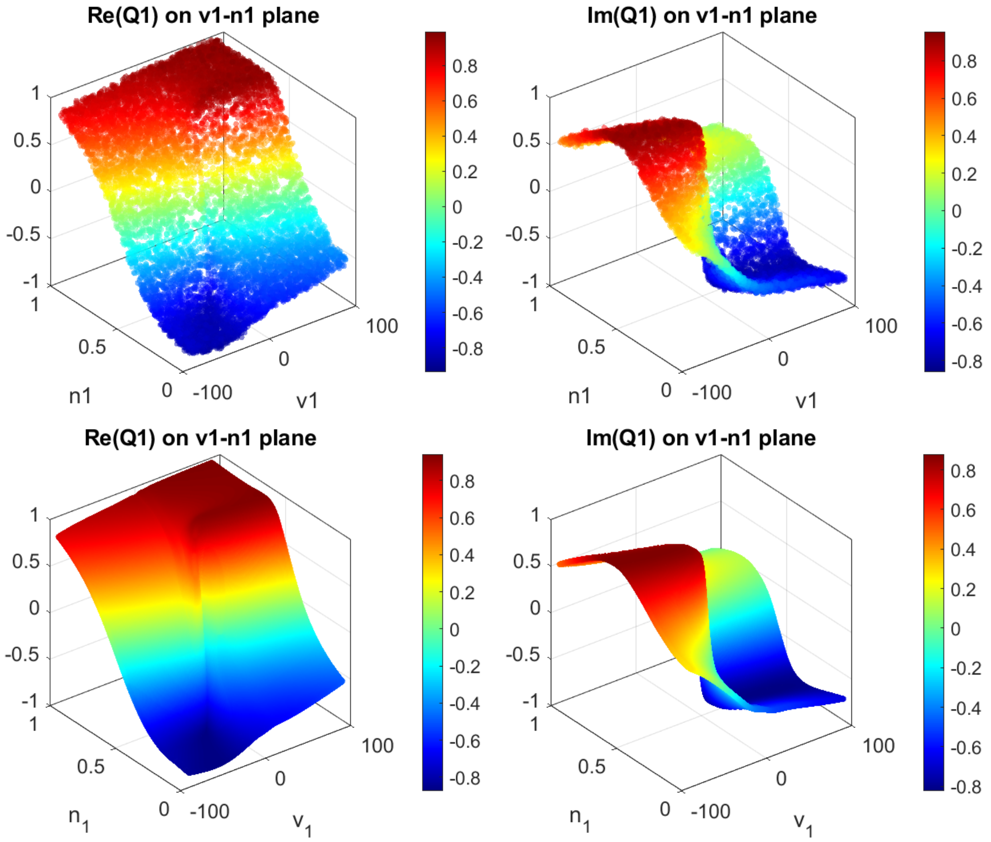


**Figure SM22.** *A projection of the 4D Q-function of (SM5.9) onto the $(v_1, n_1)$-plane, with $v_2 = 0$ and $n_2 = 0$. **Top row:** the least squares approximation at the 10,000 collocation points $\mathcal{X}$. **Bottom row:** the output of the ANN on a fine mesh, trained at the points $\mathcal{X}$ using the least squares values.*

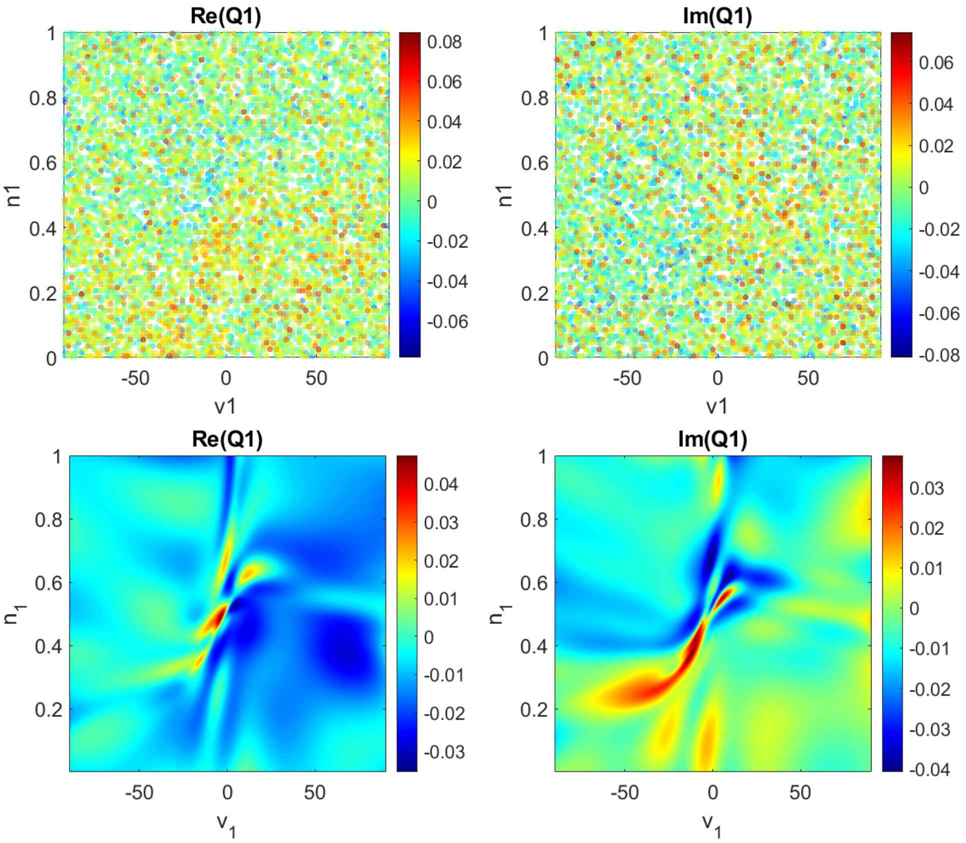


**Figure SM23.** *Heat maps of the error associated with the approximations of the 4D Q-function shown in Figure SM22.* ***Top row:*** *Difference of the least squares output and FD output at the collocation points* $\mathcal{X}$*.* ***Bottom row:*** *Difference of the ANN output trained with the least squares data and the FD output on a fine mesh. The* $L_2$ *error is* 0.0170*.*

**SM5.6. Lorenz System with Additive Noise.** As our final example, we consider a 3D Lorenz system in the chaotic regime that is subject to additive noise

$$\begin{aligned} dX &= [\sigma(Y - X)]dt + \sqrt{2D}\, dW_1(t) \\ dY &= [X(\rho - Z) - Y]dt + \sqrt{2D}\, dW_2(t) \\ dZ &= [XY - \beta Z]dt + \sqrt{2D}\, dW_3(t) \end{aligned} \tag{SM5.11}$$

where $\sigma = 10$, $\beta = 8/3$, and $\rho = 28$. The noise intensity $D$ will be varied.

We are not aware of any solution methods for the SKO eigenfunctions of (SM5.11), apart from our machine learning approach.[7] As a first step, we approximate the stationary distribution of (SM5.11) via Monte Carlo simulations. We discretize the numerical domain $\mathcal{R} = [-30, 30] \times [-40, 40] \times [-10, 60]$ into $N^3$ boxes, with $N = 100$. We choose 100,000 boxes to store in memory (according to the procedure detailed in Algorithm SM1.2), and disregard the remainder. To generate an approximation to the stationary distribution, we integrate forward in time with $dt = 0.001$ until time $T = 10{,}000$, starting from an initial condition chosen from the uniform distribution on a randomly (uniformly) chosen box. Then, we ran one trajectory and binned $N_{\text{sample}} = 100{,}000{,}000$ samples from this trajectory. We repeat this procedure for $D = 0$, $D = 0.01$, and $D = 5$. Figure SM24 shows projections onto the three coordinate planes for each case. Note that when $D = 0$ the "stationary distribution" is the well-known invariant set (the "strange attractor") of the Lorenz equations [SM19, SM13]. We apply the same procedure in the stochastic as in the deterministic case [SM11]. When $D = 0$ we obtain an approximation to the deterministic Lorenz attractor, suitable for comparison to the stationary distributions for $D > 0$.

In the following, we focus on the case when $D = 5$. We train an ANN to reproduce the stationary distribution using the 100,000 collocation points $\mathcal{X}$ and $|\mathcal{Y}|$ =700,000 reference points. The ANN was trained for 15 epochs, and iterations were divided into 64 batches, which were optimized separately to improve speed. We display the results in Figure SM25. This stationary distribution is necessary for the computation of the forward and backward eigenmodes.

We now consider the approximation of the forward eigenmode, $P_{\lambda_1}$, using our ANN approach. We run 10,000,000 trajectories and sample the forward density in 20,000 boxes at $N_t = 2000$ time-slices with timestep $dt = 0.001$ and $t_{gap} = 10$. Each realization is initialized with initial condition drawn uniformly from the box that contains the point $(10, 10, 10)$. The reference box is $\mathcal{B} = [-30, 0] \times [-30, 0] \times [-30, 20]$.

In Figure SM26, we show the decay of the forward time-dependent density in the reference box. The decaying density is fit only for time-slices $t_k$ for $k \in [500, 1700]$. Our fitting returns an estimated eigenvalue $\tilde{\lambda}_1 = -0.4107 + 7.6684i$.

We find the least squares approximation for the forward eigenfunction, including only one eigenmode in the computation. We chose the same time interval as for the eigenvalue approximation, $k \in [500, 1700]$. We also train an ANN, and show its output. The ANN was trained over 30 epochs. We used $|\mathcal{Y}|$ =500,000 reference points, and all 20,000 training points $\mathcal{X}$. Iterations were broken up into 32 batches, which were optimized separately to improve

[7] See these articles for a Koopman perspective on the deterministic Lorenz system [SM2, SM14, SM9, SM7].

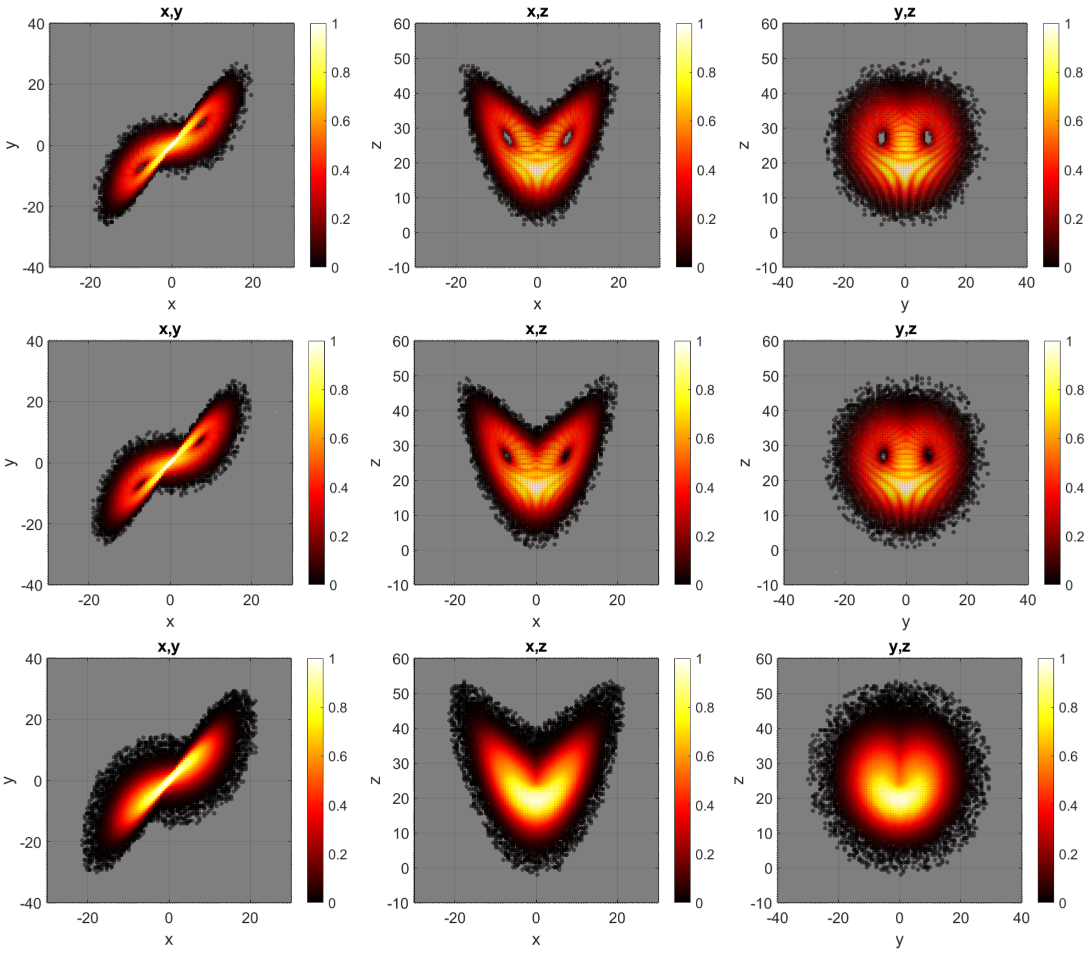


**Figure SM24.** *Monte Carlo approximations of the (unnormalized) invariant set ($D = 0$) and stationary distribution ($D > 0$) of the Lorenz system.* ***Top row:*** *$D = 0$.* ***Middle row:*** *$D = 0.01$.* ***Bottom row:*** *$D = 5$.*

speed.

Because the Lorenz system is three-dimensional, the eigenfunctions are difficult to visualize. Therefore, we first produce a 3D plot of the stationary density (computed via the ANN as described above) in Figure SM27, but keep only those points with values above a threshold of 10% of the peak density. The result is a 3D depiction of the "butterfly attractor" of the Lorenz system. We interpolate the forward eigenmode approximations from the least squares procedure and the ANN onto the butterfly attractor. Results are shown in Figure SM28. We also study the complex argument of the forward eigenfunction interpolated onto the butterfly attractor in Figure SM29. This "forward phase" is only defined near the stationary distribution, just as the complex argument associated with the *forward* eigenfunction is only well-defined on a limit-cycle in the deterministic case [SM18]. In contrast, the complex argument of the $Q$-function, i.e., the (backward) stochastic asymptotic phase, is well-defined away from the stationary distribution [SM18].

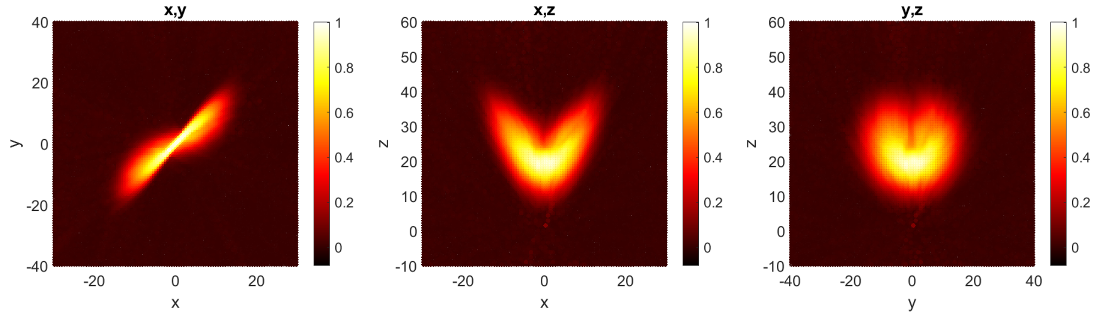


**Figure SM25.** *ANN approximation of the (unnormalized) stationary distribution of the noisy chaotic Lorenz system when $D = 5$.*

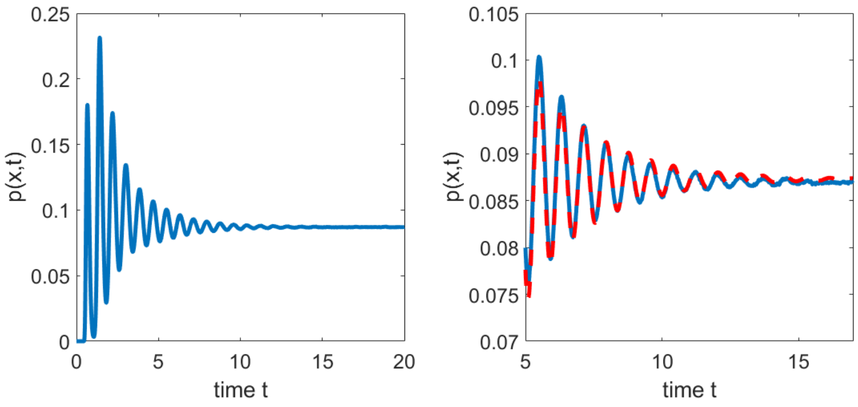


**Figure SM26.** *The decaying probability density (left) over $N_t = 2000$ time-slices for the noisy Lorenz system* (SM5.11) *with $D = 5$. We fit the decaying density using only timeslices from $t_k$ for $k \in [500, 1700]$ (red, right).*

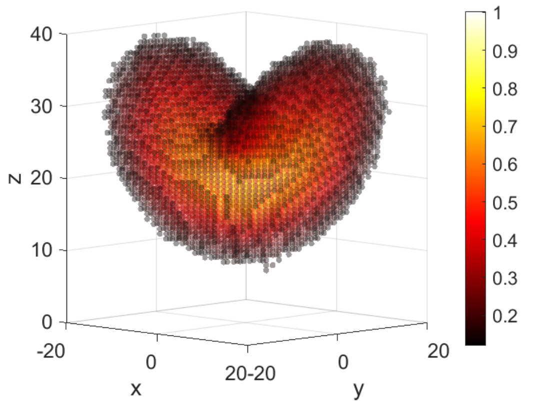


**Figure SM27.** *The butterfly attractor of the noisy Lorenz system for $D = 5$.*

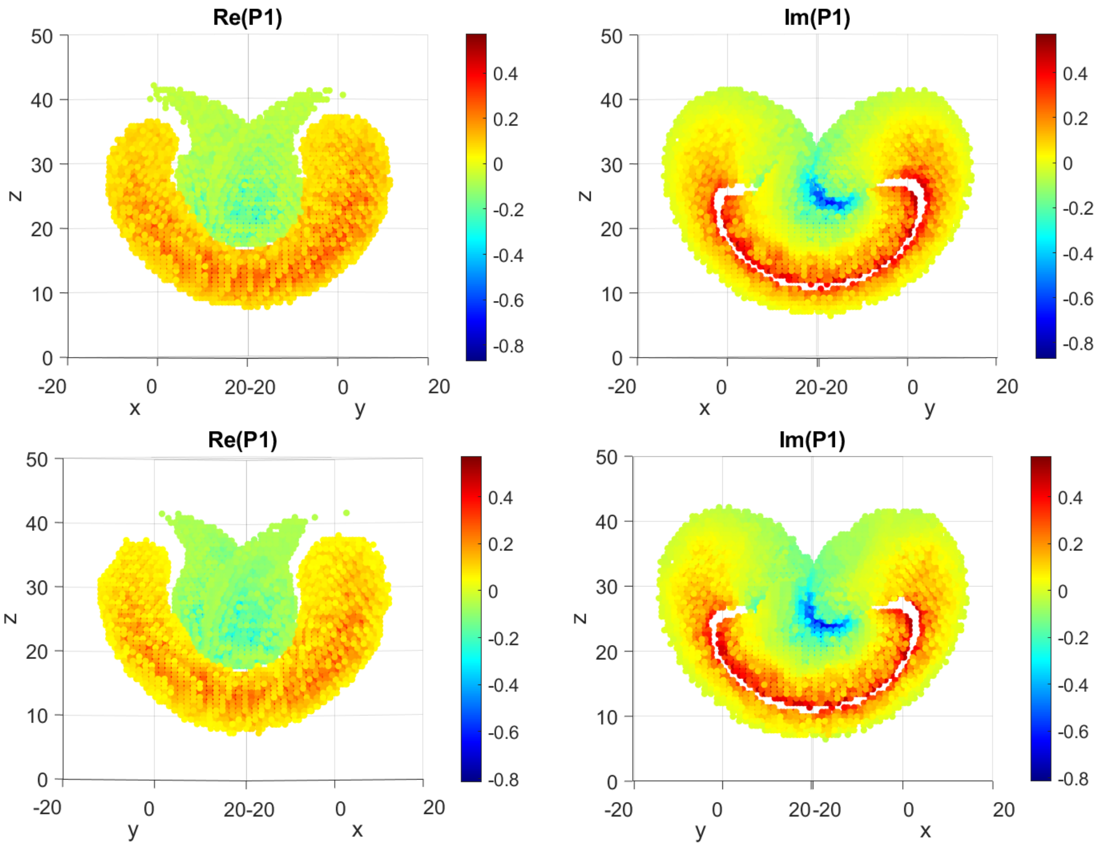


**Figure SM28.** *The slowest decaying forward eigenmode of the noisy Lorenz system.* ***Top row:*** *least squares approximation.* ***Bottom row:*** *ANN approximation. In both cases, any values falling below a threshold of* 0.05 *were disregarded to elucidate the structure of the eigenfunctions.*

Finally, we consider the $Q$-function of the noisy Lorenz system (SM5.11). We store 20,000 boxes in the domain $\mathcal{R}$. We take 20,000 initial conditions in each box, and keep track of the corresponding densities at $N_t = 900$ time-slices. We set $t_{\text{gap}} = 100$ and $dt = 0.0001$. In Figure SM30, we depict the decaying probability density corresponding to one of the boxes. Our fitting procedure estimates that $\tilde{\lambda}_1 \approx -0.4145 + 7.6709i$ taking time-slices $t_k$ with $k \in [300, 600]$.[8]

We find the least squares approximation for the $Q$-function including only one eigenmode in the computation. We chose the same time interval as for the eigenvalue approximation, $k \in [300, 600]$. We train an ANN over 40 epochs, with $|\mathcal{Y}|$ =500,000 reference points, and all 20,000 training points $\mathcal{X}$. Iterations were broken up into 128 batches, which were optimized separately to improve speed. We interpolate both the least squares and ANN solutions onto the butterfly attractor. The results are shown in Figure SM31. Figure SM32 shows the stochastic asymptotic phase $\Psi(\mathbf{x}) = \arg Q^*_{\lambda_1}(\mathbf{x})$.

[8]This estimate of $\lambda_1$ agrees to two decimal places with the estimate from the approximation of the forward eigenmodes.

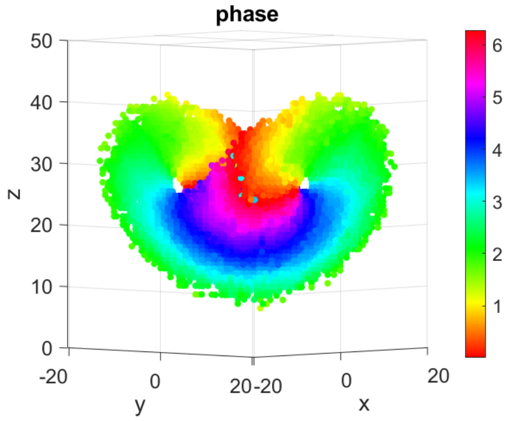


**Figure SM29.** *The complex argument of the ANN approximation of* $P_{\lambda_1}$*, interpolated onto the butterfly attractor.*

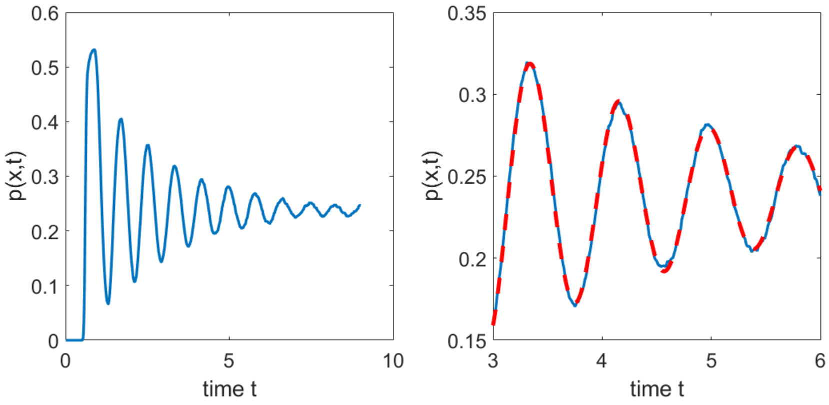


**Figure SM30.** *The decaying probability density (left) over* $N_t = 900$ *time-slices for the noisy Lorenz system* (SM5.11)*. We fit the decaying density using only timeslices from* $t_k$ *for* $k \in [300, 600]$ *(red, right).*

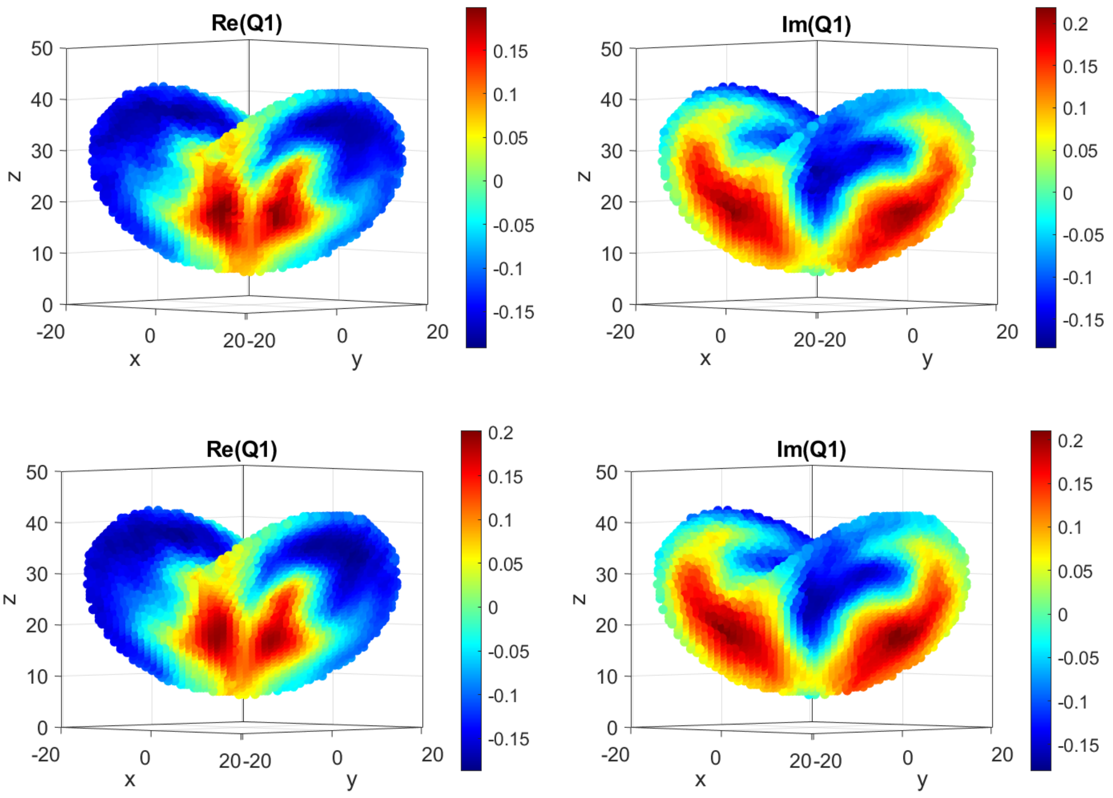


**Figure SM31.** *The Q-function of the noisy Lorenz system.* ***Top row:*** *least squares approximation.* ***Bottom row:*** *ANN approximation.*

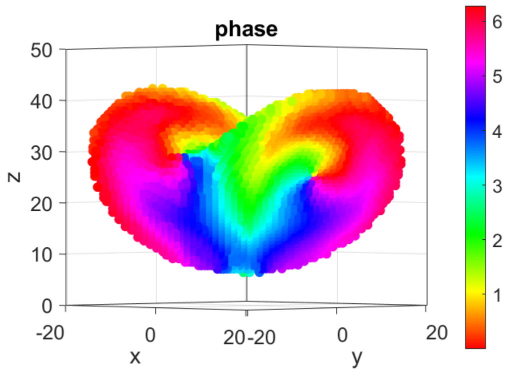


**Figure SM32.** *The "stochastic asymptotic phase" [SM18], i.e., the complex argument of the ANN approximation of $Q^*_{\lambda_1}$, interpolated onto the butterfly attractor.*

## SM6. Model Parameters.

Here, we provide details for the coupled Morris-Lecar system, whose deterministic dynamics are described by

$$\begin{aligned} C\frac{dv_1}{dt} &= I - g_L(v_1 - v_L) - g_K n_1(v_1 - v_K) - g_{CA} m_\infty(v_1)(v_1 - v_{CA}) + \kappa(v_2 - v_1) \\ C\frac{dv_2}{dt} &= I - g_L(v_2 - v_L) - g_K n_2(v_2 - v_K) - g_{CA} m_\infty(v_2)(v_2 - v_{CA}) + \kappa(v_1 - v_2) \\ \frac{dn_1}{dt} &= \alpha(v_1)(1 - n_1) - \beta(v_1)n_1 \\ \frac{dn_2}{dt} &= \alpha(v_2)(1 - n_2) - \beta(v_2)n_2 \end{aligned} \tag{SM6.1}$$

with functionals of the form

$$\begin{aligned} &\alpha(v) = \phi\frac{\cosh(\zeta_1/2)}{1+\exp(-2\zeta_1)}, \quad \beta(v) = \phi\frac{\cosh(\zeta_1/2)}{1+\exp(2\zeta_1)}, \quad m_\infty(v) = \frac{1}{2}\Big[1 + \tanh(\zeta_2)\Big], \\ &\zeta_1(v) = \frac{v - v_C}{v_D}, \quad \zeta_2(v) = \frac{v - v_A}{v_B} \end{aligned} \tag{SM6.2}$$

We choose the following parameter values

$$\begin{aligned} &I = 100,\ v_K = -84,\ v_L = -60,\ v_{CA} = 120,\ g_k = 8,\ g_L = 2,\ g_{CA} = 4.4 \\ &C = 20,\ \phi = 0.04,\ v_A = -1.2,\ v_B = 18,\ v_C = 2,\ v_D = 30 \end{aligned} \tag{SM6.3}$$

## REFERENCES


[1] J. Blechschmidt and O. G. Ernst, *Three ways to solve partial differential equations with neural networks—a review*, GAMM-Mitteilungen, 44 (2021), p. e202100006.

[2] S. L. Brunton, M. Budišić, E. Kaiser, and J. N. Kutz, *Modern koopman theory for dynamical systems*, arXiv preprint arXiv:2102.12086, (2021).

[3] C. W. Gardiner et al., *Handbook of stochastic methods*, vol. 3, springer Berlin, 1985.

[4] A. Gulli, A. Kapoor, and S. Pal, *Deep learning with TensorFlow 2 and Keras: regression, ConvNets, GANs, RNNs, NLP, and more with TensorFlow 2 and the Keras API*, Packt Publishing Ltd, 2019.

[5] W. Huang, M. Ji, Z. Liu, and Y. Yi, *Concentration and limit behaviors of stationary measures*, Physica D: Nonlinear Phenomena, 369 (2018), pp. 1–17.

[6] M. Ji, Z. Shen, and Y. Yi, *Quantitative concentration of stationary measures*, Physica D: Nonlinear Phenomena, 399 (2019), pp. 73–85.

[7] Y. Jin, L. Hou, S. Zhong, H. Yi, and Y. Chen, *Invertible koopman network and its application in data-driven modeling for dynamic systems*, Mechanical Systems and Signal Processing, 200 (2023), p. 110604.

[8] P. E. Kloeden, E. Platen, P. E. Kloeden, and E. Platen, *Stochastic differential equations*, Springer, 1992.

[9] M. Korda, M. Putinar, and I. Mezić, *Data-driven spectral analysis of the koopman operator*, Applied and Computational Harmonic Analysis, 48 (2020), pp. 599–629.

[10] M. Kreider, B. Lindner, and P. J. Thomas, *Q-functions, synchronization, and Arnold tongues for coupled stochastic oscillators*, arXiv preprint arXiv:2505.02955, (2025).

[11] A. Lasota and M. C. Mackey, *Chaos, fractals, and noise: stochastic aspects of dynamics*, vol. 97, Springer Science & Business Media, 2013.

[12] Y. Li and Y. Yi, *Systematic measures of biological networks i: Invariant measures and entropy*, Communications on Pure and Applied Mathematics, 69 (2016), pp. 1777–1811.

[13] E. N. Lorenz, *Deterministic nonperiodic flow*, Journal of Atmospheric Sciences, 20 (1963), pp. 130 – 141, https://doi.org/10.1175/1520-0469(1963)020⟨0130:DNF⟩2.0.CO;2, https://journals.ametsoc.org/view/journals/atsc/20/2/1520-0469_1963_020_0130_dnf_2_0_co_2.xml.
[14] S. E. Otto and C. W. Rowley, *Koopman operators for estimation and control of dynamical systems*, Annual Review of Control, Robotics, and Autonomous Systems, 4 (2021), pp. 59–87.
[15] A. Pérez-Cervera, B. Gutkin, P. J. Thomas, and B. Lindner, *A universal description of stochastic oscillators*, arXiv preprint arXiv:2303.03198, (2023).
[16] A. Pérez-Cervera, B. Lindner, and P. J. Thomas, *Isostables for stochastic oscillators*, Physical review letters, 127 (2021), p. 254101.
[17] Z. Shen, S. Wang, and Y. Yi, *Concentration of quasi-stationary distributions for one-dimensional diffusions with applications*, in Annales de l'Institut Henri Poincaré-Probabilités et Statistiques, vol. 60, 2024, pp. 874–903.
[18] P. J. Thomas and B. Lindner, *Asymptotic phase for stochastic oscillators*, Physical review letters, 113 (2014), p. 254101.
[19] W. Tucker, *The lorenz attractor exists*, Comptes Rendus de l'Académie des Sciences-Series I-Mathematics, 328 (1999), pp. 1197–1202.
[20] J. Zhai, M. Dobson, and Y. Li, *A deep learning method for solving fokker-planck equations*, in Mathematical and scientific machine learning, PMLR, 2022, pp. 568–597.
